# Supplementary material for: Spontaneous spin-selective structural phase transition in chiral crystals
Source: arXiv:2512.11417 source file (2026-04-18)
Supplement: Supplementary file 1 [file Supplementary_Information.pdf]

# Supplementary Information for
# "Chirality-induced spin-selective Peierls transition"

Shun Asano[1,*] and Youichi Yanase[1,†]

[1]*Department of Physics, Kyoto University, Kyoto 606-8502, Japan*

## Table of contents in Supplementary Information

**Supplementary Note 1. Details of the formulations**
1. Definition of pseudo-angular momentum
2. Selection rule of pseudo-angular momentum
3. Bir-Pikus formalism
4. Pseudo-angular momenta in the electronic bands

**Supplementary Note 2. Detailed calculations for CISSPT**
1. Notation for Green functions
2. Calculation for the renormalized phonon frequency
3. The case with explicit spin-orbit couplings
4. Gap equation of the spin-selective Peierls states
5. Resultant orders in CISSPT
6. Commensurability effect in CISSPT

**Supplementary Note 3. Derivation of collective excitations**
1. Calculation of phason and amplitudon frequencies

**Supplementary Note 4. On transverse Peierls transitions and chiral charge density waves**
1. Transverse Peierls transitions in chiral crystals
2. Collective excitations and angular momentum flow
3. Coexistence of CISSPT and winding charge density wave
4. Extension to transverse Peierls transitions in achiral crystals

**Reference**

## Supplementary Note 1. Details of the formulations.

In this Supplementary note, we explain the details of our formulation, which includes the characteristics of the pseudo-angular momentum (PAM) and the effective electron-phonon coupling (EPC). We here set $\hbar = 1$ and all the angular momenta and pseudo-angular momenta are expressed as integers or half-integers.

### 1. Definition of pseudo-angular momentum.

We consider a crystalline system preserving a $n$-fold screw symmetry $\hat{S}_n = \left[\hat{C}_n \mid \boldsymbol{c}/n\right]$ along the $z$-axis, where $\hat{C}_n$ is a $n$-fold rotation around the $z$-axis and $\boldsymbol{c}$ is a lattice vector along $z$. The Hamiltonian $\hat{H}$, $\hat{S}_n$, and the translation operator along the $z$-axis $\hat{T}_{\boldsymbol{c}}$ are all commutative:

$$[\hat{H}, \hat{S}_n] = [\hat{H}, \hat{T}_{\boldsymbol{c}}] = [\hat{S}_n, \hat{T}_{\boldsymbol{c}}] = 0.$$

Therefore, as far as the wave propagation along the $z$-axis is considered, $\hat{C}_n \boldsymbol{k} = \boldsymbol{k}$, etc., are satisfied, and the energy eigenstate can be chosen as an eigenstate of both $\hat{S}_n$ and $\hat{T}_{\boldsymbol{c}}$:

$$\hat{S}_n \psi_{\boldsymbol{k}} = \lambda^{(\mathrm{el})}_{\mathrm{S_n}} \psi_{\boldsymbol{k}},$$

where $\psi_{\boldsymbol{k}}$ is defined as symmetry-adapted Bloch eigenstates at crystal momentum $\boldsymbol{k} = (0, 0, k)$ and the irrelevant band indices are omitted for simplicity [1–4].

In spinless cases, from the property $\hat{S}_n^n = \hat{T}_{\boldsymbol{c}}$, it follows that

$$\hat{S}_n^n \psi_{\boldsymbol{k}} = \exp(-ikc)\psi_{\boldsymbol{k}},$$

and, therefore,

$$\lambda^{(\mathrm{el})}_{\mathrm{S_n}} = \exp\left(-i\frac{kc}{n} - i\frac{2\pi}{n} l_{\mathrm{PAM,el}}\right), \quad l_{\mathrm{PAM,el}} \in \mathbb{Z}_n. \tag{S.1}$$

The pseudo-angular momentum (PAM) $l_{\mathrm{PAM,el}}$ is an integer modulo $n$, which is attributed to the rotation operator included in $\hat{S}_n$ [3]. Therefore, in addition to the translational symmetry designating the crystal momentum, the eigenstates are characterized by the PAM under the screw symmetry.

In the same manner, when the degree of freedom of electron spins is included, each electronic band is labelled by the PAM $l_{\mathrm{PAM,el}}$. However, since the rotation operator $\hat{C}_n$ acts not only in real space but also in spin space, a double group is introduced to characterize the system, and $l_{\mathrm{PAM,el}}$ becomes a half-integer [1]. Then, we construct the symmetry-adapted Bloch function categorized by $l_{\mathrm{PAM,el}} \in \mathbb{Z}_n/2$ as

$$\psi_{\boldsymbol{k},\, l_{\mathrm{PAM}}}(\boldsymbol{r}) = \sum_{\sigma} e^{ikz} e^{im^{(\mathrm{orb})}_{\boldsymbol{k}}\Phi} u_{\boldsymbol{k},\, m^{(\mathrm{orb})},\, \sigma}(\rho, \Phi, z) \left|\sigma\right\rangle,$$

where $\left|\sigma\right\rangle$ denotes the spin state ($\left|\uparrow\right\rangle, \left|\downarrow\right\rangle$), $\Phi$ is the azimuthal angle within the $xy$ plane, and $u_{\boldsymbol{k},\sigma}(\boldsymbol{r}) = u_{\boldsymbol{k},\sigma}(\rho, \Phi, z)$ is a periodic function with lattice periodicity, written in cylindrical coordinates:

$$u_{\boldsymbol{k},\sigma}(\rho, \Phi - 2\pi/n, z - c/n) = u_{\boldsymbol{k},\sigma}(\rho, \Phi, z).$$

Here, $m^{(\mathrm{orb})}$ represents the phase factor that arises from the screw operator. Under this formulation, because the screw operator acts on both real space coordinates and spin, the wave function is transformed as

$$\begin{aligned}
\hat{S}_n \psi_{\boldsymbol{k}, l_{\mathrm{PAM}}}(\boldsymbol{r}) &= \sum_{\sigma\sigma'} e^{ik(z-c/n)} e^{im^{(\mathrm{orb})}_{\boldsymbol{k}}(\Phi - 2\pi/n)} u_{\boldsymbol{k},\sigma}(\rho, \Phi - 2\pi/n, z - c/n) \left[\hat{U}_{\mathrm{spin}}(C_n)\right]_{\sigma\sigma'} \left|\sigma'\right\rangle \\
&= e^{-ikc/n} e^{ikz} \sum_{\sigma\sigma'} e^{-2\pi i m^{(\mathrm{orb})}_{\boldsymbol{k}}/n} e^{im^{(\mathrm{orb})}_{\boldsymbol{k}}\Phi} u_{\boldsymbol{k},\sigma}(\rho, \Phi, z) \left[\hat{U}_{\mathrm{spin}}(C_n)\right]_{\sigma\sigma'} \left|\sigma'\right\rangle \\
&= \sum_{\sigma} \exp\left(-i\frac{kc}{n} - i\frac{2\pi}{n}(m^{(\mathrm{orb})}_{\boldsymbol{k}} + m^{(\mathrm{spin})}_{\boldsymbol{k}})\right) e^{ikz} e^{im^{(\mathrm{orb})}_{\boldsymbol{k}}\Phi} u_{\boldsymbol{k},\sigma}(\rho, \Phi, z) \left|\sigma\right\rangle,
\end{aligned}$$

where $\hat{U}_{\mathrm{spin}}(C_n) = \exp(-i\frac{2\pi}{n}\frac{\sigma_z}{2})$ is the SU(2) spin rotation matrix corresponding to $\hat{C}_n$, and we used

$$\hat{U}_{\mathrm{spin}}(C_n) \left|\sigma\right\rangle = e^{-i\frac{2\pi}{n} m^{(\mathrm{spin})}_{\boldsymbol{k}}} \left|\sigma\right\rangle, \tag{S.2}$$

with $m^{(\rm spin)} = \pm 1/2$ for $|\uparrow\rangle$ and $|\downarrow\rangle$, respectively. Therefore, the electron PAM can be decomposed into $m^{(\rm orb)}$ and $m^{(\rm spin)}$; the former originates from the real space coordinate dependence of the Bloch function and the latter from the spin space. In other words, the total electron PAM is generally preserved modulo $n$ in each eigenstate:

$$l_{\rm PAM,el} = m_{\boldsymbol{k}}^{(\rm orb)} + m_{\boldsymbol{k}}^{(\rm spin)}. \tag{S.3}$$

In general, although their sum modulo $n$ remains a good quantum number, $m^{(\rm orb)}$ and $m^{(\rm spin)}$ are not individually conserved. However, at wave vectors where the electronic spin is regarded a good quantum number, it is expected that $m^{(\rm orb)}$ and $m^{(\rm spin)}$ can be approximately treated separately. This applies not only to systems with negligible spin-orbit coupling (SOC), but also to cases where SOC preserves the spin direction either locally or globally, such as in $\hat{H}_{\rm SOI} = \alpha_{\rm SO}\boldsymbol{k}\cdot\boldsymbol{\sigma}$ [5–8].

It is important to note that the electron PAM is fundamentally different from the orbital angular momenta. The latter refers to the characteristics of atomic orbitals or the rotational motion of electrons, which are largely independent of the global crystal symmetry. Meanwhile, the former is a quantum number determined solely by the screw symmetry of the crystal. Hence, it is the PAM rather than the angular momenta that plays a significant role in phenomena involving the screw symmetry, e.g., selection rules in chiral crystals with helical structures. However, it is expected that the features of atomic orbitals underlie those of PAM because each atomic orbital constitutes the PAM in a way that the symmetry of the crystal adopts.

In the same manner, the phonon PAM is defined at crystal momentum $\boldsymbol{q} = (0, 0, q)$ by the eigenvalue of $\hat{S}_n$ [9–12]:

$$\hat{S}_n \mathbf{u}_{\mathbf{q}}(\mathbf{r}) = \lambda_{S_n}^{(\rm ph)} \mathbf{u}_{\mathbf{q}}(\mathbf{r}).$$

As long as considering the phonon propagation along the $z$-axis, the explicit expression becomes

$$\begin{aligned}\hat{S}_n \mathbf{u}_{\mathbf{q}}(\mathbf{r}) &= \left[\hat{C}_n \boldsymbol{\epsilon}_{\mathbf{q}}\right] \zeta_{\mathbf{q}} \exp\left(i\mathbf{q}\cdot[\hat{C}_n|\mathbf{c}/n]^{-1}\mathbf{r}\right) \\ &= \left[\hat{C}_n \boldsymbol{\epsilon}_{\mathbf{q}}\right] \zeta_{\mathbf{q}} \exp\left(i(\hat{C}_n\mathbf{q})\cdot\mathbf{r} - i(\hat{C}_n\mathbf{q})\cdot\frac{\mathbf{c}}{n}\right) \\ &= \left[\hat{C}_n \boldsymbol{\epsilon}_{\mathbf{q}}\right] \zeta_{\mathbf{q}} \exp\left(iqz - i\frac{qc}{n}\right),\end{aligned}$$

where we used

$$[\hat{C}_n|\mathbf{c}/n]^{-1} = [\hat{C}_n^{-1}| - \hat{C}_n^{-1}\mathbf{c}/n].$$

The eigenvalue of $\left[\hat{C}_n \boldsymbol{\epsilon}_{\mathbf{q}}\right]$ corresponding to the discrete rotation is related to $\exp\left(-i\frac{2\pi}{n} l^s_{\rm PAM,ph}\right)\boldsymbol{\epsilon}_{\mathbf{q}}$ with the discrete integer $l^s_{\rm PAM,ph}$. Therefore,

$$\hat{S}_n \mathbf{u}_{\mathbf{q}}(\mathbf{r}) = \exp\left(-i\frac{qc}{n} - i\frac{2\pi}{n} l^s_{\rm PAM,ph}\right)\mathbf{u}_{\mathbf{q}}(\mathbf{r}), \tag{S.4}$$

holds, where the spin part $l^s_{\rm PAM,ph} \in \mathbb{Z}_n$ originates from the local atomic rotation. Note that, in the context of phonon PAM, the phase factor $\exp(-iqc/n)$ is usually written as $\exp(-i\frac{2\pi}{n} l^o_{\rm PAM,ph})$, where $l^o_{\rm PAM,ph}$ is interpreted as the orbital component of phonon PAM. The total phonon PAM is then written as the sum $l^s_{\rm PAM,ph} + l^o_{\rm PAM,ph}$. In contrast, in this article, we refer to the spin part merely as phonon PAM in order to avoid confusion with the designation in electronic systems.

**2. Selection rule of pseudo-angular momentum.**

In the previous section, we introduced the PAM defined by screw symmetry. Here, we provide an overview of the conservation laws of the PAM between the initial and final states through the interaction process. Hereafter, as in the main text, we consider wave vectors such as $\boldsymbol{k} = (0, 0, k)$, and the index $z$ is omitted for simplicity.

The screw symmetry of the crystal conserves the total PAM, just as the lattice periodicity conserves the total crystal momentum. It is not the angular momentum but the PAM that is strictly conserved. This is similar to the situation where the discrete angular momentum, rather than the angular momentum, is conserved under rotation symmetry. Expressed in a more detailed form, when the interaction Hamiltonian $\hat{H}_{\rm int}$ is invariant with respect to screw symmetry $\hat{S}_n$;

$$\hat{S}_n^{-1}\hat{H}_{\rm int}\hat{S}_n = \hat{H}_{\rm int},$$

the total PAM of all elementary excitations involved is conserved modulo $n$. One of the well-known examples is the selection rule for the optical transition process [9, 10, 13, 14], where the total PAM of the phonon and the circularly polarized light is conserved. Moreover, the crystal momentum is conserved between the initial and final states;

$$\boldsymbol{k}_{i,1} + \boldsymbol{k}_{i,2} + \cdots = \boldsymbol{k}_{f,1} + \boldsymbol{k}_{f,2} + \cdots,$$

where $i(f)$ means the initial (final) state. This relation makes factors such as $\exp(-ikc/n)$ included in the PAM ignorable because they are always cancelled out:

$$\exp(-i\frac{k_{i,1}c}{n})\exp(-i\frac{k_{i,2}c}{n})\cdots=\exp(-i\frac{k_{f,1}c}{n})\exp(-i\frac{k_{f,2}c}{n})\cdots.$$

Therefore, the selection rule is usually written by the discrete part of PAM, e.g., $l_{\mathrm{PAM,\,el}}$ or $l^{s}_{\mathrm{PAM,\,ph}}$ that we defined above.

As another example, the same argument can be applied to the EPC. In this case, the phonon PAM and the electron PAM are involved in the selection rule [2]. Thus, the following constraints are imposed on the interaction Hamiltonian by the screw symmetry alone, in the process of phonon creation or annihilation:

$$l_{\mathrm{PAM,\,el}}+l^{s}_{\mathrm{PAM,\,ph}}=l'_{\mathrm{PAM,\,el}}\qquad\mathrm{mod}\ n,$$

or equivalently

$$m^{(\mathrm{orb})}_{\boldsymbol{k}}+m^{(\mathrm{spin})}_{\boldsymbol{k}}+l^{s}_{\mathrm{PAM,\,ph}}=m'^{(\mathrm{orb})}_{\boldsymbol{k}+\boldsymbol{q}}+m'^{(\mathrm{spin})}_{\boldsymbol{k}+\boldsymbol{q}}\qquad\mathrm{mod}\ n.$$

However, it is not clear whether the EPC induces spin flips in electrons. In other words, the spin PAM $m^{(\mathrm{spin})}_{\boldsymbol{k}}$ could be independently preserved and the selection rule does not necessarily involve both orbital and spin components $m^{(\mathrm{orb})}_{\boldsymbol{k}}$ and $m^{(\mathrm{spin})}_{\boldsymbol{k}}$. This is because, when the electron PAM is well separated into these components and the EPC only includes contributions from the lattice displacement, exchange between the phonon and electron PAM occurs sorely in the orbital components.

In the following sections, we consider a more general form of the EPC Hamiltonian based on previous research [15, 16]. Starting from the Hamiltonian that explicitly includes the spin-orbit coupling, we will derive the effective EPC, of which the selection rule includes both $m^{(\mathrm{spin})}_{\boldsymbol{k}}$ and $m^{(\mathrm{orb})}_{\boldsymbol{k}}$.

**3. Bir-Pikus formalism.**

In the elementary formulation, the Fröhlich Hamiltonian is commonly used to describe the EPC, incorporating only the effect of the periodic potential modulated by lattice displacements. However, the modified lattice potential can exert a crucial influence on electrons via the SOC. Several previous studies derived the EPC that takes into account both the modification of the periodic potential and the variation in the SOC strength induced by phonons [15, 17–21]. In particular, Luo and Dai qualitatively discussed the EPC under rotational symmetry [15], where the effects of phonon-induced lattice displacements on electrons are fully considered. We therefore extend this theory to systems under screw symmetry and qualitatively derive the EPC between chiral phonons and electrons.

The essence of Ref. [15] is that the deformation of the lattice potential due to phonons is treated beyond the regular perturbation theory because a generic deformed lattice potential no longer has the same periodicity as the original one in general. Hence, the coordinates are transformed so that the periodicity in the new coordinate system, which incorporates phonon displacements, coincides with the unstrained system in the original one. Subsequently, derivation of the effective EPC is achieved by performing the usual perturbation theory. We here briefly follow the same approach while replacing the features associated with rotational symmetry with those with screw symmetry.

We also start from the single-electron Hamiltonian, which respects the lattice symmetry:

$$\hat{H}_0=\frac{\hat{\boldsymbol{p}}^2}{2m_e}+V_0(\hat{\boldsymbol{r}})+\xi_{\mathrm{SO}}\hat{\boldsymbol{p}}\cdot(\hat{\boldsymbol{\sigma}}\times\nabla V_0(\hat{\boldsymbol{r}}))\,,\tag{S.5}$$

where we assume the periodic potential is screw symmetric satisfying $\hat{S}_n^{-1}V_0(\hat{\boldsymbol{r}})\hat{S}_n=V_0(\hat{\boldsymbol{r}})$. The total Hamiltonian, therefore, also satisfies $\hat{S}_n^{-1}\hat{H}_0\hat{S}_n=\hat{H}_0$. The local strain operator $\hat{\varepsilon}$ in terms of the phonon displacement is calculated by $\hat{\varepsilon}_{lm}=\partial_m\hat{\mathbf{u}}_l$. This strain transforms the electron's operators and wave numbers up to the linear order as follows.

$$\begin{aligned}\hat{\boldsymbol{r}}&\to\hat{\boldsymbol{r}}+\hat{\boldsymbol{\varepsilon}}\hat{\boldsymbol{r}},\\ \hat{\boldsymbol{p}}&\to\hat{\boldsymbol{p}}-\hat{\boldsymbol{\varepsilon}}\hat{\boldsymbol{p}},\\ \boldsymbol{k}&\to\boldsymbol{k}-\boldsymbol{\varepsilon}\boldsymbol{k}.\end{aligned}$$

Accordingly, the Hamiltonian is transformed in the deformed coordinate, and the margin corresponds to the part of EPC:

$$\hat{H}_0\to\hat{H}_0+\hat{H}_{\mathrm{int}}.$$

According to the detailed calculations in Ref. [15], the EPC Hamiltonian $\hat{H}_{\mathrm{int}}$ can be expressed using a certain rank-2 tensor operator and the strain operator as follows.

$$\begin{aligned}\hat{H}_{\mathrm{int}}&=-\frac{1}{m_e}\left(\hat{\boldsymbol{p}}+\xi_{\mathrm{SO}}(\hat{\boldsymbol{\sigma}}\times\nabla V_0)\right)_i\hat{\boldsymbol{\varepsilon}}_{ij}\hat{\boldsymbol{p}}_j-\xi_{\mathrm{SO}}(\hat{\boldsymbol{p}}\times\hat{\boldsymbol{\sigma}})_i\hat{\boldsymbol{\varepsilon}}_{ij}\partial_jV_0+V_{ij}\hat{\boldsymbol{\varepsilon}}_{ij}+\xi_{\mathrm{SO}}\left[\hat{\boldsymbol{\sigma}}\times(\hat{\boldsymbol{\varepsilon}}_{ij}\nabla V_{ij})\right]\cdot\hat{\boldsymbol{p}}\\&\equiv\hat{\boldsymbol{\varepsilon}}_{ij}\hat{\mathcal{V}}_{ij}+\mathcal{O}(q^2),\end{aligned}\tag{S.6}$$

where

$$V_{ij} = \lim_{\varepsilon \to 0} \frac{V_\varepsilon\left((1+\hat{\boldsymbol{\varepsilon}})\boldsymbol{r}\right) - V_0(\boldsymbol{r})}{\hat{\boldsymbol{\varepsilon}}_{ij}}. \tag{S.7}$$

We are now able to use safely the conventional perturbation theory and obtain the total effective Hamiltonian and the corresponding Bloch function, which satisfy

$$\begin{aligned}\hat{H}^{(\text{eff})}_{\boldsymbol{k}}\, \tilde{u}_{\boldsymbol{k}}(\boldsymbol{r}) &= E_{\boldsymbol{k}} \tilde{u}_{\boldsymbol{k}}(\boldsymbol{r}), \\ \tilde{\psi}_{\boldsymbol{k}}(\boldsymbol{r}) &= e^{i\boldsymbol{k}\cdot\boldsymbol{r}} u_{\boldsymbol{k}}\left((\mathbf{1}+\boldsymbol{\varepsilon})\boldsymbol{r}\right) \equiv e^{i\boldsymbol{k}\cdot\boldsymbol{r}} \tilde{u}_{\boldsymbol{k}}\left(\boldsymbol{r}\right).\end{aligned}$$

Through further calculations with $k \cdot p$ perturbation, we obtain the following expression, where we focused on the dominant contribution of the EPC term $\hat{H}_{\text{ep}}$ up to the zeroth order of $\boldsymbol{k}$ and the first order of $\boldsymbol{q}$.

$$\begin{aligned}\hat{H}^{(\text{eff})}_{\boldsymbol{k}} &= \hat{H}_{0,\,\boldsymbol{k}} + \hat{H}_{\text{ep}}, \\ \hat{H}_{0,\,\boldsymbol{k}} &\equiv e^{-i\boldsymbol{k}\cdot\boldsymbol{r}} \hat{H}_0 e^{i\boldsymbol{k}\cdot\boldsymbol{r}} \\ &= \frac{\hbar^2 k^2}{2m_e} + \frac{\hbar}{m_e}\boldsymbol{k}\cdot\left[\hat{\boldsymbol{p}} + \xi_{\text{SO}}\left(\hat{\boldsymbol{\sigma}} \times \nabla V_0(\boldsymbol{r})\right)\right] + \hat{H}_0, \\ \hat{H}_{\text{ep}} &= \hat{\boldsymbol{\varepsilon}}_{ij} \hat{\mathcal{V}}_{ij}.\end{aligned}$$

So far, we have not specified the coordinate system strictly. Here, since we are interested in chiral phonons, we introduce the chiral basis and rewrite all vector components accordingly. Moreover, when we focus on the phonon propagation along the chiral axis, the strain tensor components $\hat{\boldsymbol{\varepsilon}}_{iz}$ $(i = x, y)$ are significant. Then we rewrite the local strain in the chiral basis as follows,

$$\begin{aligned}\hat{\boldsymbol{\varepsilon}}_\pm &\equiv \frac{1}{\sqrt{N_{\text{i}}}} \sum_q iq \sqrt{\frac{\hbar}{2M_{\text{i}}\omega_{q,\pm}}} (\hat{b}_{q,\pm} + \hat{b}^\dagger_{-q,\mp}) e^{iqz}, \\ \hat{\boldsymbol{\varepsilon}}_0 &\equiv \frac{1}{\sqrt{N_{\text{i}}}} \sum_q iq \sqrt{\frac{\hbar}{2M_{\text{i}}\omega_{q,0}}} (\hat{b}_{q,0} + \hat{b}^\dagger_{-q,0}) e^{iqz},\end{aligned}$$

and accordingly, we also redefine the spherical components $\hat{\mathcal{V}}_0, \hat{\mathcal{V}}_\pm$ so that the EPC Hamiltonian becomes $\hat{H}_{\text{ep}} = \hat{\boldsymbol{\varepsilon}}_0 \hat{\mathcal{V}}_0 + \hat{\boldsymbol{\varepsilon}}_+ \hat{\mathcal{V}}_- + \hat{\boldsymbol{\varepsilon}}_- \hat{\mathcal{V}}_+$. Therefore, we finally reach the matrix elements of the EPC Hamiltonian:

$$\begin{aligned}\langle \psi_{k,l_{\text{PAM, el}}} | \, \hat{\boldsymbol{\varepsilon}}_0 \hat{\mathcal{V}}_0 \, | \psi_{k',l'_{\text{PAM, el}}} \rangle &= iq \sqrt{\frac{\hbar}{2N_{\text{i}} M_{\text{i}} \omega_{q,0}}} (\hat{b}_{q,0} + \hat{b}^\dagger_{-q,0}) \langle u_{k,l_{\text{PAM, el}}} | \, \hat{\mathcal{V}}_0 \, | u_{k',l_{\text{PAM, el}}} \rangle \; \delta(k'+q,\, k)\, \delta(l'_{\text{PAM, el}},\, l_{\text{PAM, el}}) \\ &\equiv \frac{g^{(0)}(k, q, l_{\text{PAM, el}}, , l'_{\text{PAM, el}})}{\sqrt{N_{\text{i}}}} iq\, \hat{\zeta}_{q,0}\, \delta(k'+q,\, k)\, \delta(l'_{\text{PAM, el}},\, l_{\text{PAM, el}}), \\ \langle \psi_{k,l_{\text{PAM, el}}} | \, \hat{\boldsymbol{\varepsilon}}_\pm \hat{\mathcal{V}}_\mp \, | \psi_{k',l'_{\text{PAM, el}}} \rangle &= iq \sqrt{\frac{\hbar}{2N_{\text{i}} M_{\text{i}} \omega_{q,\pm}}} (\hat{b}_{q,\pm} + \hat{b}^\dagger_{-q,\mp}) \langle u_{k,l_{\text{PAM, el}}} | \, \hat{\mathcal{V}}_\mp \, | u_{k',l_{\text{PAM, el}}} \rangle \\ &\qquad \times \delta(k'+q,\, k)\, \delta(l'_{\text{PAM, el}} \pm 1,\, l_{\text{PAM, el}}) \\ &\equiv \frac{g^{(\pm)}(k, q, l_{\text{PAM, el}}, l'_{\text{PAM, el}})}{\sqrt{N_{\text{i}}}}\, iq\, \hat{\zeta}_{q,\pm}\, \delta(k'+q,\, k)\, \delta(l'_{\text{PAM, el}} \pm 1,\, l_{\text{PAM, el}}).\end{aligned}$$

Note that our notation slightly differs from that of Ref. [15] because we have defined the components of the phonon displacement in chiral coordinates.

In the above derivation, there are three points worth mentioning. To begin with, as previously mentioned, the total PAM as well as the crystal momentum are conserved as a consequence of screw symmetry alone. This was mentioned in the previous study [2], where the total PAM excluding the electron spin contribution is conserved because the EPC arising from the modified hopping strength was considered. It is also pointed out that, in each phonon mode with a specific PAM, the longitudinal and transverse components are mixed [2, 9, 22–27]. However, the phonon PAM approximately coincides with the phonon angular momentum in the long-wavelength regime. In some models [22, 23], this correspondence remains accurate even up to half of the Brillouin zone (BZ). Therefore, for brevity, in the main text, we do not explicitly distinguish between the angular momentum and

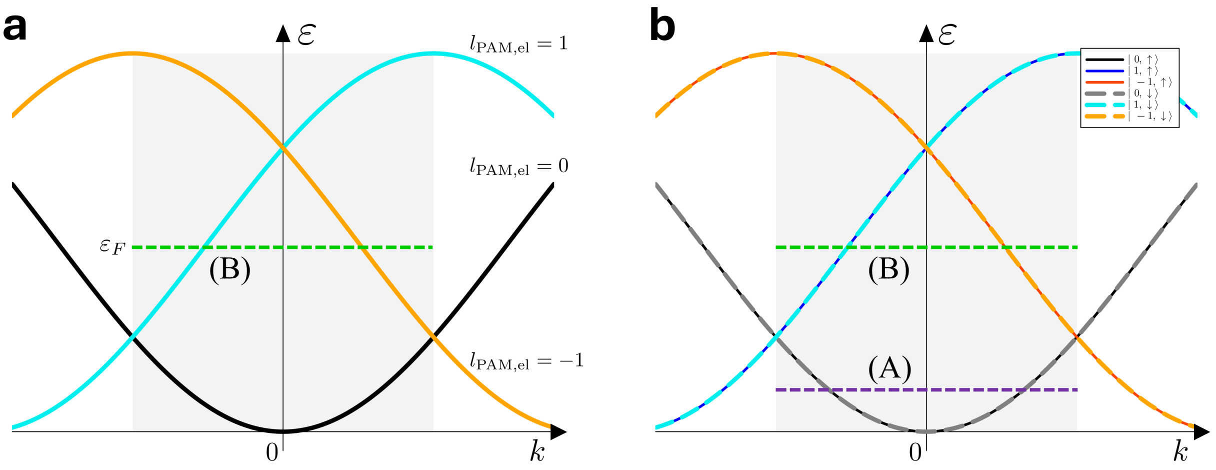


Supplementary Figure S1. **Electronic band structures classified by pseudo-angular momentum with $\hat{S}_3$ symmetry** [1]. **a**, The electronic bands for spinless case, where the bands are labelled by integer PAM. **b**, The electronic bands for spinful case with negligible spin–orbit coupling, where PAM is a half-integer. Two representative Fermi levels are indicated by the purple dashed line (A) and green dashed line (B). The electronic bands are shown in the extended zone scheme and the gray rectangle represents the reduced BZ folded by the $\hat{S}_3$ symmetry.

PAM unless necessary, and rewrite $l_{\mathrm{PAM,\,ph}} = 0, \pm 1 \to l^{(\mathrm{ph})}_{z,L} = 0,\ l^{(\mathrm{ph})}_{z,\lambda} = \lambda\ (\lambda = \pm 1)$. Accordingly, the phonon Hamiltonian is written as the sum of all branches:

$$\hat{H}_{\mathrm{ph}} = \sum_q \hbar\omega_{q,\mathrm{L}} \hat{b}^\dagger_{q,\mathrm{L}} \hat{b}_{q,\mathrm{L}} + \sum_{q,\lambda} \hbar\omega_{q,\lambda} \hat{b}^\dagger_{q,\lambda} \hat{b}_{q,\lambda}.$$

Next, it is impractical to determine the coupling coefficients $g^{(0)}(k, q, l_{\mathrm{PAM,\,el}})$, $g^{(\pm)}(k, q, l_{\mathrm{PAM,\,el}}, l'_{\mathrm{PAM,\,el}})$ in realistic materials. In this study, we assume

$$g^{(0)}(k, q, l_{\mathrm{PAM,\,el}}, l'_{\mathrm{PAM,\,el}}) = g_L,$$
$$g^{(\pm)}(k, q, l_{\mathrm{PAM,\,el}}, l'_{\mathrm{PAM,\,el}}) = g_T,$$

with the constants $g_L$ and $g_T$. This simplification is justified by the fact that our analysis focuses on qualitative features, and the difference in magnitude between $g^{(+)}(k, q, l_{\mathrm{PAM,\,el}}, l'_{\mathrm{PAM,\,el}})$ and $g^{(-)}(k, q, l_{\mathrm{PAM,\,el}}, l'_{\mathrm{PAM,\,el}})$ has only a minor effect due to the intrinsic splitting of the phonon branches $\omega_{q,\pm}$.

The last point is that we assumed a Hamiltonian with SOC as the starting point for the derivation. This allows us to safely conclude that total PAM conservation includes the electron spin component; namely, $l^s_{\mathrm{PAM,\,ph}}$, $m^{(\mathrm{orb})}$, and $m^{(\mathrm{spin})}$ are all intertwined. This type of EPC is called spin-orbit assisted electron-phonon coupling in some studies [20, 21]. Its physical interpretation is given as follows [18]. The change in the periodic potential associated with the lattice displacements, i.e., the modulation of $\nabla V_0(\hat{\boldsymbol{r}})$, induces an additional local electric field. This field has the SOC-like effect, causing $l_{\mathrm{PAM,\,ph}}$, $m^{(\mathrm{orb})}_{\boldsymbol{k},\sigma}$, and $m^{(\mathrm{spin})}_{\boldsymbol{k},\sigma}$ to all hybridize. Therefore, it is expected that the strong SOC in an electronic system favors CISSPT. However, it is not certain whether this type of EPC is weak in a system with a weak electronic SOC. This is because even if the intrinsic field $\nabla V_0(\hat{\boldsymbol{r}})$ is sufficiently small, such terms as $V_{ij}$ in Eq. (S.6) could become large enough. A more quantitative evaluation of their details is expected in future studies.

With keeping the above points in mind, in the main text, we assume a simple SOC Hamiltonian for the electronic system, since our main interest is the role of chiral phonons. Specifically, we consider a parabolic approximation or a spin-diagonal Hamiltonian $\hat{H}_{\mathrm{SO}} = \alpha_{\mathrm{SO}}\, \boldsymbol{k} \cdot \boldsymbol{\sigma}$ as simple models. In these cases, the electronic PAM is simplified as $l_{\mathrm{PAM,\,el}} = m_{\mathrm{orb}} + \sigma$. Therefore, we eventually obtain the EPC for each branch.

$$\hat{H}^{(\mathrm{L})}_{\mathrm{ep}} = \frac{1}{\sqrt{N_{\mathrm{i}}}} \sum_{\boldsymbol{k},q} \sum_{s,s',m_{\mathrm{orb}},m'_{\mathrm{orb}}} iqg_L \hat{c}^\dagger_{k+q,s,m_{\mathrm{orb}}} \hat{c}_{k,s',m'_{\mathrm{orb}}} \hat{\zeta}_{q,\mathrm{L}}\, \delta_{m_{\mathrm{orb}}+s,\, m'_{\mathrm{orb}}+s'}, \tag{S.8}$$

$$\hat{H}^{(\mathrm{T})}_{\mathrm{ep}} = \frac{1}{\sqrt{N_{\mathrm{i}}}} \sum_{\boldsymbol{k},q} \sum_{s,s',m_{\mathrm{orb}},m'_{\mathrm{orb}}} \sum_{\lambda=\pm} iqg_T \hat{c}^\dagger_{k+q,s,m_{\mathrm{orb}}} \hat{c}_{k,s',m'_{\mathrm{orb}}} \hat{\zeta}_{q,\lambda}\, \delta_{m_{\mathrm{orb}}+s,\, m'_{\mathrm{orb}}+s'+l^{\mathrm{ph}}_{z,\lambda}}. \tag{S.9}$$

**4. Pseudo-angular momenta in the electronic bands.**
Figure S1 illustrates how the PAM classifies electronic bands with the three-fold screw symmetry and the possible Peierls instabilities. Figure S1a shows the spinless case, where the PAM takes integer values. On the other hand, Figure S1b shows the spinful case with negligible SOC, in which the PAM is a half-integer and the spin remains a good quantum number. In this situation, the electronic bands are labelled by $l_{\mathrm{PAM,el}} = m_{\boldsymbol{k}}^{(\mathrm{orb})} + s$.

When the Fermi level intersects the band with $m_{\mathrm{orb}} = 0$ corresponding to (A), i.e., the orbital contributions are not involved, the conservation law of PAM in the EPC reduces to the relation $s + l_{\mathrm{PAM,ph}} = s'$. Only the electron spin and the phonon PAM participate in this process, and the resulting instability corresponds to the CISSPT discussed in the main text and Supplementary Notes 2-3. By contrast, when the Fermi level lies in the bands with non-zero $m_{\mathrm{orb}}$ as shown by (B), such that electron spin is not changed, the Peierls instability couples the states with $m_{\mathrm{orb}} = \pm 1$. In this case, PAM conservation is fulfilled through the orbital component of the electron and the phonon PAM, leading to a transverse Peierls transition and a winding charge density wave as described in Supplementary Note 4.

In essence, Fig. S1 highlights that the nature of the Peierls instability, whether spin-selective Peierls states or winding CDW states are realized, is determined by whether the spin or the orbital component of the electronic PAM, or both of them participate in the conservation law at the Fermi level.

## Supplementary Note 2. Detailed calculations for CISSPT.

In this Supplementary note, we show the details of calculations and add information for the basic properties of chirality-induced spin-selective Peierls transitions.

### 1. Notations for Green functions.

In this section, we briefly describe the basic notation for later calculations using the Green function [28]. Regarding the phonon Green function, the expectation value $\langle \hat{\zeta}_{q,\eta}\hat{\zeta}_{q',\eta'}\rangle$ is finite only for time-reversal paired indices, that is, when $q' = -q$ and $\eta' = -\eta$; otherwise, it vanishes. Therefore, the phonon Green function is defined as

$$\mathscr{D}(q,\eta,\tau-\tau') = -\langle T\big(\hat{b}_{q,\eta}(\tau) + \hat{b}^\dagger_{-q,-\eta}(\tau)\big)\big(\hat{b}_{-q,-\eta}(\tau') + \hat{b}^\dagger_{q,\eta}(\tau')\big)\rangle,$$

where $\tau$ is the imaginary time. We omit the interaction and Heisenberg representation indicators for brevity. Each mode can be written down in detail as

$$\begin{aligned}
\mathscr{D}^{(0)}_{\mathrm{L}}(q,\tau-\tau') &\equiv \mathscr{D}^{(0)}(q,L,\tau-\tau') \\
&= -e^{-\hbar\omega_{q,L}(\tau-\tau')}\left[\Theta(\tau-\tau')(1+n(\hbar\omega_{q,L})) + \Theta(\tau'-\tau)n(\hbar\omega_{q,L})\right] \\
&\quad - e^{\hbar\omega_{-q,L}(\tau-\tau')}\left[\Theta(\tau-\tau')n(\hbar\omega_{-q,L}) + \Theta(\tau'-\tau)(1+n(\hbar\omega_{-q,L}))\right], \\
\mathscr{D}^{(0)}_{\mathrm{T}}(q,\lambda,\tau-\tau') &\equiv \mathscr{D}^{(0)}(q,\lambda,\tau-\tau') \\
&= -e^{-\hbar\omega_{q,\lambda}(\tau-\tau')}\left[\Theta(\tau-\tau')(1+n(\hbar\omega_{q,\lambda})) + \Theta(\tau'-\tau)n(\hbar\omega_{q,\lambda})\right] \\
&\quad - e^{\hbar\omega_{-q,-\lambda}(\tau-\tau')}\left[\Theta(\tau-\tau')n(\hbar\omega_{-q,-\lambda}) + \Theta(\tau'-\tau)(1+n(\hbar\omega_{-q,-\lambda}))\right].
\end{aligned}$$

We then perform a Fourier transformation on the phonon Green function with respect to the Matsubara frequency:

$$\begin{aligned}
\mathscr{D}^{(0)}_{\mathrm{L}}(q,i\omega_m) &\equiv \int_0^\beta d\tau\, \mathscr{D}^{(0)}_{\mathrm{L}}(q,\tau)e^{i\omega_m\tau} \\
&= \frac{2\hbar\omega_{q,L}}{(i\omega_m)^2 - (\hbar\omega_{q,L})^2}, \\
\mathscr{D}^{(0)}_{\mathrm{T}}(q,\lambda,i\omega_m) &\equiv \int_0^\beta d\tau\, \mathscr{D}^{(0)}_{\mathrm{T}}(q,\lambda,\tau)e^{i\omega_m\tau} \\
&= \frac{2\hbar\omega_{q,\lambda}}{(i\omega_m)^2 - (\hbar\omega_{q,\lambda})^2},
\end{aligned}$$

where we used $\omega_{-q,L} = \omega_{q,L}$ and $\omega_{-q,-\lambda} = \omega_{q,\lambda}$, and $\omega_m = 2\pi m/\beta$ denote the bosonic Matsubara frequencies.

On the other hand, the electron Green function is defined as

$$\mathscr{G}_{ss'}(k,\tau-\tau') = -\langle T\hat{c}_{k,s}(\tau)\hat{c}^\dagger_{k,s'}(\tau')\rangle.$$

When the electron Hamiltonian is spin-diagonal, it becomes

$$\mathscr{G}^{(0)}_{ss'}(k,i\epsilon_n) = \frac{1}{i\epsilon_n - \xi_{k,s}}\delta_{s,s'},$$

where $\epsilon_n = (2n+1)\pi/\beta$ are the fermionic Matsubara frequencies.

Accordingly, the electron-phonon coupling for CISSPT (see the main text) is given by the following expression in the interaction representation.

$$\begin{aligned}
\hat{H}^{(\mathrm{L})}_{\mathrm{ep}}(\tau) &= \frac{1}{\sqrt{N_{\mathrm{i}}}}\sum_{\boldsymbol{k},q,s,s'} g^{(\mathrm{L})}_{s,s'}(q)\hat{c}^\dagger_{k+q,s}(\tau)\hat{c}_{k,s'}(\tau)\big(\hat{b}_{q,L}(\tau) + \hat{b}^\dagger_{-q,L}(\tau)\big), \\
\hat{H}^{(\mathrm{T})}_{\mathrm{ep}}(\tau) &= \frac{1}{\sqrt{N_{\mathrm{i}}}}\sum_{\boldsymbol{k},q,\lambda,s,s'} g^{(\mathrm{T})}_{s,s'}(q,\lambda)\hat{c}^\dagger_{k+q,s}(\tau)\hat{c}_{k,s'}(\tau)\big(\hat{b}_{q,\lambda}(\tau) + \hat{b}^\dagger_{-q,-\lambda}(\tau)\big),
\end{aligned}$$

and we define the vertex coefficient for the following calculation as follows.

$$g^{(\mathrm{L})}_{s,s'}(q) = iqg_{\mathrm{L}}\sqrt{\frac{\hbar}{2M_{\mathrm{i}}\omega_{q,L}}}(\hat{\sigma}_0)_{ss'}, \tag{S.10}$$

$$g^{(\mathrm{T})}_{s,s'}(q,\lambda) = iqg_{\mathrm{T}}\sqrt{\frac{\hbar}{2M_{\mathrm{i}}\omega_{q,\lambda}}}(\hat{\sigma}_\lambda)_{ss'}. \tag{S.11}$$

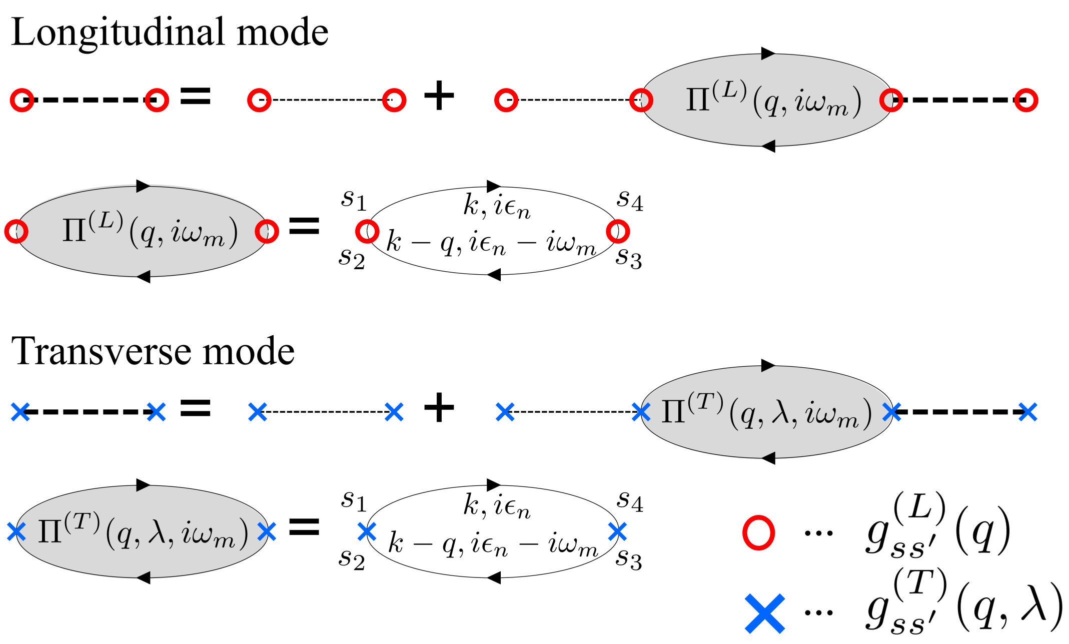


Supplementary Figure S2. **Feynman diagram for the calculation of the renormalized phonon frequency.** The red circles represent the vertex part for $\hat{H}^{(\mathrm{L})}_{\mathrm{ep}}$ while the blue crosses for $\hat{H}^{(\mathrm{T})}_{\mathrm{ep}}$.

**2. Calculations for the renormalized phonon frequency.**
We describe in detail the method for calculating the renormalized phonon frequencies. We begin by deriving the general form of the phonon self-energy [29]. The renormalized phonon frequency under the random phase approximation (RPA) can be evaluated from the Feynman diagrams shown in Fig. S2. The Green functions for the dressed phonons, which incorporate electronic screening, satisfy the following Dyson equations:

$$\begin{aligned}\mathscr{D}_{\mathrm{L}}(q,i\omega_m) =& \mathscr{D}^{(0)}_{\mathrm{L}}(q,i\omega_m) + \mathscr{D}^{(0)}_{\mathrm{L}}(q,i\omega_m)\Pi^{(\mathrm{L})}(q,i\omega_m)\mathscr{D}_{\mathrm{L}}(q,i\omega_m),\\ \mathscr{D}_{\mathrm{T}}(q,\lambda,i\omega_m) =& \mathscr{D}^{(0)}_{\mathrm{T}}(q,\lambda,i\omega_m) + \mathscr{D}^{(0)}_{\mathrm{T}}(q,\lambda,i\omega_m)\Pi^{(\mathrm{T})}(q,\lambda,i\omega_m)\mathscr{D}_{\mathrm{T}}(q,\lambda,i\omega_m).\end{aligned}$$

Therefore,

$$\begin{aligned}\mathscr{D}^{-1}_{\mathrm{L}}(q,i\omega_m) =& \mathscr{D}^{(0)}_{\mathrm{L}}(q,i\omega_m)^{-1} - \Pi^{(\mathrm{L})}(q,i\omega_m),\\ \mathscr{D}^{-1}_{\mathrm{T}}(q,\lambda,i\omega_m) =& \mathscr{D}^{(0)}_{\mathrm{T}}(q,\lambda,i\omega_m)^{-1} - \Pi^{(\mathrm{T})}(q,\lambda,i\omega_m).\end{aligned}$$

Under the RPA and the Migdal approximation, the phonon self-energy is

$$\begin{aligned}\Pi^{(\mathrm{L})}(q,i\omega_m) =& \frac{k_BT}{N_{\mathrm{i}}}\sum_{k,i\epsilon_n}\sum_{s_1s_2s_3s_4} g^{(\mathrm{L})}_{s_1s_2}(q)g^{(\mathrm{L})}_{s_3s_4}(-q)\mathscr{G}^{(0)}_{s_4s_1}(k,i\epsilon_n)\mathscr{G}^{(0)}_{s_2s_3}(k-q,i\epsilon_n-i\omega_m),\\ \Pi^{(\mathrm{T})}(q,\lambda,i\omega_m) =& \frac{k_BT}{N_{\mathrm{i}}}\sum_{k,i\epsilon_n}\sum_{s_1s_2s_3s_4} g^{(\mathrm{T})}_{s_1s_2}(q,\lambda)g^{(\mathrm{T})}_{s_3s_4}(-q,-\lambda)\mathscr{G}^{(0)}_{s_4s_1}(k,i\epsilon_n)\mathscr{G}^{(0)}_{s_2s_3}(k-q,i\epsilon_n-i\omega_m).\end{aligned}$$

Substituting Eqs. (S.10) and (S.11) yields

$$\begin{aligned}\Pi^{(\mathrm{L})}(q,i\omega_m) =& \frac{k_BT}{N_{\mathrm{i}}}\sum_{k,i\epsilon_n}\sum_{s}\frac{\hbar q^2 g_{\mathrm{L}}^2}{2M_{\mathrm{i}}\omega_{q,L}}\mathscr{G}^{(0)}_{ss}(k,i\epsilon_n)\mathscr{G}^{(0)}_{ss}(k-q,i\epsilon_n-i\omega_m) \equiv \frac{\hbar q^2 g_{\mathrm{L}}^2}{2M_{\mathrm{i}}\omega_{q,L}}\chi_{zz}(q,i\omega_m),\\ \Pi^{(\mathrm{T})}(q,+,i\omega_m) =& \frac{k_BT}{N_{\mathrm{i}}}\sum_{k,i\epsilon_n}\frac{2\hbar q^2 g_{\mathrm{T}}^2}{M_{\mathrm{i}}\omega_{q,+}}\mathscr{G}^{(0)}_{\uparrow\uparrow}(k,i\epsilon_n)\mathscr{G}^{(0)}_{\downarrow\downarrow}(k-q,i\epsilon_n-i\omega_m) \equiv \frac{2\hbar q^2 g_{\mathrm{T}}^2}{M_{\mathrm{i}}\omega_{q,+}}\chi_{+-}(q,i\omega_m),\\ \Pi^{(\mathrm{T})}(q,-,i\omega_m) =& \frac{k_BT}{N_{\mathrm{i}}}\sum_{k,i\epsilon_n}\frac{2\hbar q^2 g_{\mathrm{T}}^2}{M_{\mathrm{i}}\omega_{q,-}}\mathscr{G}^{(0)}_{\downarrow\downarrow}(k,i\epsilon_n)\mathscr{G}^{(0)}_{\uparrow\uparrow}(k-q,i\epsilon_n-i\omega_m) \equiv \frac{2\hbar q^2 g_{\mathrm{T}}^2}{M_{\mathrm{i}}\omega_{q,-}}\chi_{-+}(q,i\omega_m).\end{aligned}$$

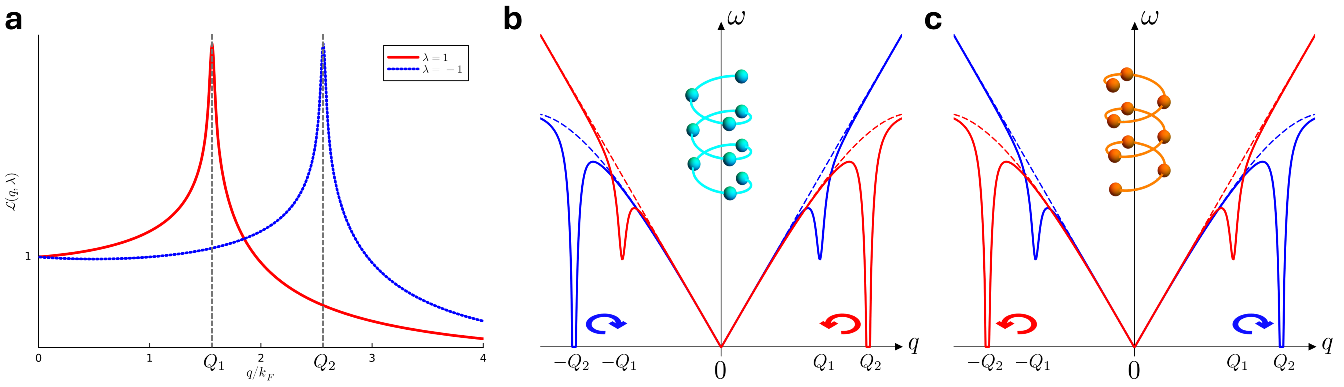


Supplementary Figure S3. **Softening of chiral phonons with explicit spin-orbit coupling.** **a**, Dimensionless Lindhard function $\tilde{L}_\lambda(q,\lambda)$ for $\alpha_{\rm SO}k_F/\varepsilon_F = 1$, showing logarithmic singularities at wave vectors $Q_1$ and $Q_2$. **b**, Schematic illustration of the phonon dispersion for the LH crystal. Chiral phonon branches $\lambda = \pm 1$ exhibit Kohn anomalies at distinct wave vectors $Q_1$ and $Q_2$. **c**, Schematic illustration of the phonon dispersion for the RH crystal. The correspondence between phonon chirality and nesting vectors is reversed relative to the LH crystal.

Here, $\chi_{zz}, \chi_{+-}, \chi_{-+}$ correspond to individual susceptibility functions, and their explicit forms are given by the Lindhard function:

$$\frac{k_B T}{N_{\rm i}} \sum_{k,i\epsilon_n} \mathscr{G}^{(0)}_{ss}(k, i\epsilon_n)\mathscr{G}^{(0)}_{s's'}(k-q, i\epsilon_n - i\omega_m) = \frac{1}{N_{\rm i}}\sum_k \frac{f(\varepsilon_{k-q,s'}) - f(\varepsilon_{k,s})}{i\omega_m + \varepsilon_{k-q,s'} - \varepsilon_{k,s}}. \tag{S.12}$$

By performing the analytic continuation $i\omega_m \to \hbar\omega + i\delta$, the renormalized phonon frequencies correspond to the poles of the renormalized phonon Green functions, and therefore, they are determined by the condition $\mathscr{D}_L^{-1}(q,\hbar\omega+i\delta) = 0$, $\mathscr{D}_T^{-1}(q,\lambda,\hbar\omega+i\delta) = 0$, where

$$\mathscr{D}_L^{-1}(q,\hbar\omega+i\delta) = \frac{1}{2\hbar\omega_{q,L}}\left[(\hbar\omega+i\delta)^2 - (\hbar\omega_{q,L})^2\left(1 + \frac{2}{\hbar\omega_{q,L}}\Pi^{(\rm L)}(q,\omega)\right)\right], \tag{S.13}$$

$$\mathscr{D}_T^{-1}(q,\lambda,\hbar\omega+i\delta) = \frac{1}{2\hbar\omega_{q,\lambda}}\left[(\hbar\omega+i\delta)^2 - (\hbar\omega_{q,\lambda})^2\left(1 + \frac{2}{\hbar\omega_{q,\lambda}}\Pi^{(\rm T)}(q,\lambda,\omega)\right)\right]. \tag{S.14}$$

As usual, the phonon energy scale is assumed to be sufficiently small relative to the Fermi energy. Therefore, the frequency dependence of the phonon self-energies is negligible, and the renormalized phonon frequencies are obtained as

$$(\hbar\tilde{\omega}_{q,L})^2 = (\hbar\omega_{q,L})^2\left(1 + \frac{2}{\hbar\omega_{q,L}}{\rm Re}\,\Pi^{(\rm L)}(q,0)\right),$$
$$(\hbar\tilde{\omega}_{q,\lambda})^2 = (\hbar\omega_{q,\lambda})^2\left(1 + \frac{2}{\hbar\omega_{q,\lambda}}{\rm Re}\,\Pi^{(\rm T)}(q,\lambda,0)\right).$$

### 3. The case with explicit electronic spin-orbit couplings.

In the main text and Methods, the formulations in the previous section are used to obtain the renormalized phonon frequencies with spin-degenerate electrons. We here show that the same argument can be extended to the case with the electron Hamiltonian including the explicit SOC term. Let us consider the following electron Hamiltonian as the model case.

$$\hat{H}_{\rm e} = \left(\frac{\hbar^2 k^2}{2m_e} - \epsilon_F\right)\hat{\sigma}_0 + \alpha_{\rm SO}\boldsymbol{k}\cdot\hat{\boldsymbol{\sigma}} = \left(\frac{\hbar^2 k^2}{2m_e} - \epsilon_F\right)\hat{\sigma}_0 + \alpha_{\rm SO}k\hat{\sigma}_z,$$

that is, the eigenenergy is

$$\epsilon_{k,s} = \frac{\hbar^2 k^2}{2m_e} + \alpha_{SO}ks.$$

Although the sign of the SOC coupling constant $\alpha_{\rm SO}$ depends on the material, it is generally flipped between opposite enantiomorphs [5–8].

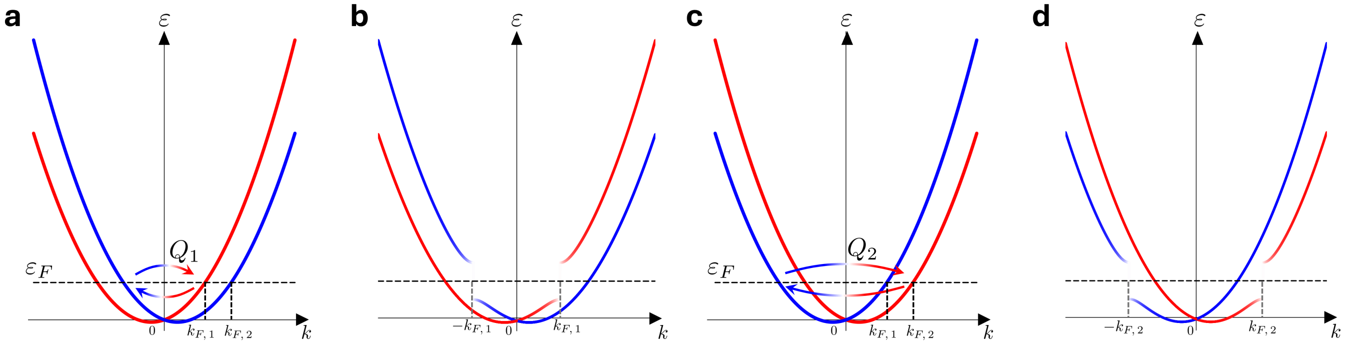


Supplementary Figure S4. **Spin-selective Peierls states in the LH crystal with explicit spin-orbit coupling. a** and **b**, Case of positive $\alpha_{\rm SO}$ and the soft phonons $(Q_1,+)$ and $(-Q_1,-)$. The nesting vector $Q_1$ couples the electronic subbands with $(-k_{F,1},\downarrow)$ and $(k_{F,1},\uparrow)$, where $k_{F,1}=Q_1/2$. **c** and **d**, Case of negative $\alpha_{\rm SO}$ and the soft phonons $(Q_2,+)$ and $(-Q_2,-)$, corresponding to Fig. S3b. The electronic subbands with $(-k_{F,2},\downarrow)$ and $(k_{F,2},\uparrow)$ are coupled, where $k_{F,2}=Q_2/2$.

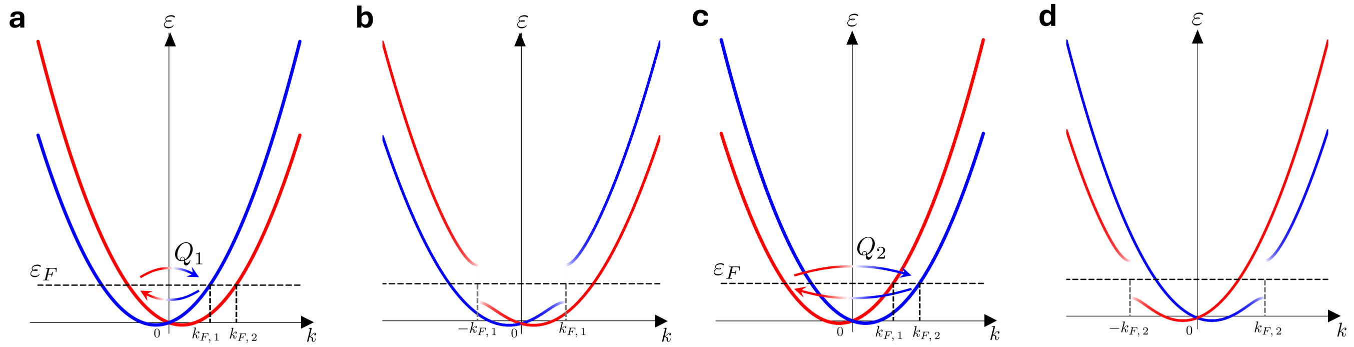


Supplementary Figure S5. **Spin-selective Peierls states in the RH crystal with explicit spin-orbit coupling. a** and **b**, Case of negative $\alpha_{\rm SO}$ and the soft phonons $(Q_1,-)$ and $(-Q_1,+)$. The nesting vector $Q_1$ couples the electronic subbands with $(-k_{F,1},\uparrow)$ and $(k_{F,1},\downarrow)$. **c** and **d**, Case of positive $\alpha_{\rm SO}$ and the soft phonons $(Q_2,-)$ and $(-Q_2,+)$, corresponding to Fig. S3c. The electronic subbands with $(-k_{F,2},\uparrow)$ and $(k_{F,2},\downarrow)$ are coupled.

Then, the phonon self-energy with respect to the chiral phonon becomes

$$\begin{aligned}\Pi^{(\mathrm{T})}(q,+,i\omega_m) =&\frac{2\hbar q^2 g_{\mathrm{T}}^2}{M_{\mathrm{i}}\omega_{q,+}}\chi_{+-}(q,i\omega_m)\\ =&\frac{2\hbar q^2 g_{\mathrm{T}}^2}{M_{\mathrm{i}}\omega_{q,+}}\frac{1}{N_{\mathrm{i}}}\sum_k \frac{f(\epsilon_{k-q,\downarrow})-f(\epsilon_{k,\uparrow})}{i\omega_m+\epsilon_{k-q,\downarrow}-\epsilon_{k,\uparrow}},\\ \Pi^{(\mathrm{T})}(q,-,i\omega_m) =&\frac{2\hbar q^2 g_{\mathrm{T}}^2}{M_{\mathrm{i}}\omega_{q,-}}\chi_{-+}(q,i\omega_m)\\ =&\frac{2\hbar q^2 g_{\mathrm{T}}^2}{M_{\mathrm{i}}\omega_{q,-}}\frac{1}{N_{\mathrm{i}}}\sum_k \frac{f(\epsilon_{k-q,\uparrow})-f(\epsilon_{k,\downarrow})}{i\omega_m+\epsilon_{k-q,\uparrow}-\epsilon_{k,\downarrow}}.\end{aligned}$$

Therefore, the renormalized phonon frequency of each chirality is obtained as

$$(\hbar\tilde{\omega}_{q,\pm})^2 =(\hbar\omega_{q,\pm})^2\left(1-\Lambda\tilde{\mathcal{L}}_{\pm}(q,0)\right),$$

where $\Lambda$ is a dimensionless electron-phonon coupling constant described in Eq. (S.37) below, and we define the dimensionless Lindhard function:

$$\tilde{\mathcal{L}}_\lambda(q,\omega)=-\frac{1}{N_{\mathrm{i}}}\sum_k\sum_{s,s'}\mathrm{Re}\left[\frac{f(\epsilon_{k-q,s})-f(\epsilon_{k,s'})}{\hbar\omega+i0+\epsilon_{k-q,s}-\epsilon_{k,s'}}\delta(s'-s-\lambda)\right]. \tag{S.15}$$

Figure S3a shows the $q$ dependence of $\tilde{\mathcal{L}}(q,\lambda) \equiv \tilde{\mathcal{L}}_\lambda(q,\omega=0)$ at low temperatures $k_BT/\epsilon_F \ll 1$. We set $\alpha_{\rm SO}k_F/\epsilon_F = 1$. The wave vectors at which divergence occurs are given by

$$Q_1/k_F = -\frac{\alpha_{SO}k_F}{2\varepsilon_F} + \sqrt{\left(\frac{\alpha_{SO}k_F}{2\varepsilon_F}\right)^2 + 4}, \tag{S.16}$$

$$Q_2/k_F = \frac{\alpha_{SO}k_F}{2\varepsilon_F} + \sqrt{\left(\frac{\alpha_{SO}k_F}{2\varepsilon_F}\right)^2 + 4}. \tag{S.17}$$

Accordingly, the soft modes are modulated, and as shown in Figs. S3b and S3c, the chiral phonons with each chirality exhibit the Kohn anomaly at different wave vectors $Q_1$ and $Q_2$.

If we alternatively set $\alpha_{\rm SO}k_F/\epsilon_F = -1$, the wave vectors of anomaly, $Q_1$ and $Q_2$, are switched, and thereby the handedness of frozen phonons is reversed from those shown in Fig. S3. Because the sign of the SOC coupling constant $\alpha_{\rm SO}$ is opposite between different enantiomorphs, the handedness of frozen phonons is closely related to the handedness of crystals. Furthermore, because the sign of $\alpha_{\rm SO}$ can alter depending on the environment even for a fixed enantiomorph, it introduces an additional variety of Kohn anomaly: the SOC parameter determines which of the two nesting vectors, $Q_1$ or $Q_2$, governs the Peierls instability. The combination of crystal handedness and the sign of $\alpha_{\rm SO}$ yields four distinct possibilities for the feasible Peierls states. In the RH crystal corresponding to Fig. S3c, the cases with negative and positive $\alpha_{\rm SO}$ are illustrated in Figs. S5a,b and Figs. S5c,d, respectively. In contrast, for the LH crystal, the same consideration applies with the handedness reversed, as shown in Fig. S4. These four cases exhaust the possible spin-selective Peierls states stabilized in the presence of explicit electronic SOC.

In any case, by treating the spin-split bands as independent subbands, the analysis is a natural extension of the spin-degenerate case, and the same conclusions are obtained. Furthermore, as long as the spin remains a well-defined quantum number at the Fermi level, the argument herein is expected to apply to other types of SOC such as the Rashba SOC [30, 31].

**4. Gap equation of spin-selective Peierls states.**

In this section, we note the detailed calculations for incommensurate spin-selective Peierls states. We consider spin-degenerate electron bands under the parabolic approximation for simplicity. The energy dispersion in the parent phase is given by

$$\boldsymbol{\xi}_k = \left(\frac{\hbar^2k^2}{2m_e} - \varepsilon_F\right)\delta_{ss'}. \tag{S.18}$$

Under these approximations, the minimal Hamiltonian relevant to the CISSPT is given by

$$\mathcal{H} = \sum_{0<k} \begin{bmatrix} c^\dagger_{k,\uparrow} & c^\dagger_{k-2k_F,\downarrow}\end{bmatrix} \begin{bmatrix} \dfrac{\hbar^2k^2}{2m_e} - \varepsilon_F & \Delta \\ \Delta^* & \dfrac{\hbar^2(k-2k_F)^2}{2m_e} - \varepsilon_F \end{bmatrix} \begin{bmatrix} c_{k,\uparrow} \\ c_{k-2k_F,\downarrow}\end{bmatrix}. \tag{S.19}$$

Diagonalizing this matrix, the quasiparticle energy bands below the transition temperature, for $k > 0$ measured relative to the Fermi level are obtained as

$$E_\pm(k) = \frac{\varepsilon_k + \varepsilon_{k-2k_F}}{2} \pm \sqrt{\left(\frac{\varepsilon_k - \varepsilon_{k-2k_F}}{2}\right)^2 + |\Delta|^2} - \varepsilon_F, \tag{S.20}$$

where

$$\varepsilon_k = \frac{\hbar^2k^2}{2m_e}. \tag{S.21}$$

For $k < 0$, the band dispersion can be obtained by replacing $k \to -k$ in the above expression. Thus, in the extended zone scheme, the band structure is composed of the following branches:

$$\begin{aligned} &E_-(k) && (0 < k < k_F), \\ &E_+(k) && (k_F < k), \\ &E_-(-k) && (-k_F < k < 0), \\ &E_+(-k) && (k < -k_F). \end{aligned}$$

Let the unitary matrix used for diagonalization be defined via

$$\begin{aligned}\begin{bmatrix}\hat{\alpha}_{k,-}\\ \hat{\alpha}_{k,+}\end{bmatrix} &= U^{-1}(k)\begin{bmatrix}\hat{c}_{k,\uparrow}\\ \hat{c}_{k-2k_F,\downarrow}\end{bmatrix}\\ &= U^{\dagger}(k)\begin{bmatrix}\hat{c}_{k,\uparrow}\\ \hat{c}_{k-2k_F,\downarrow}\end{bmatrix}\\ &= \begin{bmatrix}u_{11}^*(k) & u_{21}^*(k)\\ u_{12}^*(k) & u_{22}^*(k)\end{bmatrix}\begin{bmatrix}\hat{c}_{k,\uparrow}\\ \hat{c}_{k-2k_F,\downarrow}\end{bmatrix}.\end{aligned} \tag{S.22}$$

Then, the expectation value of the spin along the $z$-axis in the diagonalized bands is given by

$$E_-(k): \quad s_z(k) = \frac{\hbar}{2}\left(|u_{11}(k)|^2 - |u_{21}(k)|^2\right) = \frac{\hbar}{2}\left(|\boldsymbol{u}_1^-(k)|^2 - |\boldsymbol{u}_2^-(k)|^2\right), \tag{S.23}$$

$$E_+(k): \quad s_z(k) = \frac{\hbar}{2}\left(|u_{12}(k)|^2 - |u_{22}(k)|^2\right) = \frac{\hbar}{2}\left(|\boldsymbol{u}_1^+(k)|^2 - |\boldsymbol{u}_2^+(k)|^2\right), \tag{S.24}$$

where $\boldsymbol{u}^{\pm}(k)$ denotes the eigenvector corresponding to the eigenvalue $E_{\pm}(k)$.

We now focus on the fact that the electronic ordered state is primarily governed by the states near the Fermi energy. We restrict our analysis to the vicinity of $(k_F, \uparrow)$ and $(-k_F, \downarrow)$, which are the states relevant to the CISSPT. The energy dispersion can be approximated near these points as

$$\begin{aligned}\xi_k &= \hbar v_F(k - k_F) \qquad \text{for } k \simeq k_F,\\ \xi_k &= -\hbar v_F(k + k_F) \quad \text{for } k \simeq -k_F.\end{aligned} \tag{S.25}$$

By expressing the Peierls gap as $\Delta = |\Delta| e^{i\phi}$, separating its amplitude and phase, the Hamiltonian becomes

$$\mathcal{H} = \sum_{0<k}\begin{bmatrix}c_{k,\uparrow}^{\dagger} & c_{k-2k_F,\downarrow}^{\dagger}\end{bmatrix}\begin{bmatrix}\xi_k & \Delta\\ \Delta^* & -\xi_k\end{bmatrix}\begin{bmatrix}c_{k,\uparrow}\\ c_{k-2k_F,\downarrow}\end{bmatrix}, \tag{S.26}$$

and the eigenvalues and eigenvectors of this matrix are given by

$$\begin{aligned}E_{\pm}(k) &= \pm\sqrt{\xi_k^2 + |\Delta|^2} \equiv \pm E_k,\\ U(k) &= \begin{bmatrix}u(k) & v^*(k)\\ -v(k) & u(k)\end{bmatrix},\\ u(k) &= \sqrt{\frac{1}{2}\left(1 - \frac{\xi_k}{E_k}\right)},\\ v(k) &= e^{-i\phi}\sqrt{\frac{1}{2}\left(1 + \frac{\xi_k}{E_k}\right)}.\end{aligned}$$

Accordingly, the expectation value of the density wave associated with the CISSPT is calculated as

$$\begin{aligned}\left\langle\sum_k \hat{c}_{k+Q,\uparrow}^{\dagger}\hat{c}_{k,\downarrow}\right\rangle &= \left\langle\hat{S}_{-Q}^{(+)}\right\rangle = \left\langle\hat{S}_{Q}^{(-)}\right\rangle^*\\ &= \sum_k\left\langle\left[u(k)\hat{\alpha}_{k,-}^{\dagger} + v(k)\hat{\alpha}_{k,+}^{\dagger}\right]\left[-v(k)\hat{\alpha}_{k,-} + u(k)\hat{\alpha}_{k,+}\right]\right\rangle\\ &= -\sum_k\frac{\Delta^*(Q)}{2E_k}\left(1 - 2f(E_k)\right),\end{aligned} \tag{S.27}$$

where $f(E_k)$ is the Fermi distribution function.

On the other hand, let us denote the phonon conjugate momentum by $\hat{\pi}_{q,\lambda}$. Then the phonon Hamiltonian is expressed as

$$\begin{aligned}\hat{H}_{\text{ph}} &= \sum_{q,\lambda}\hbar\omega_{q,\lambda}b_{q,\lambda}^{\dagger}b_{q,\lambda}\\ &= \sum_{q,\lambda}\left[\frac{M_{\text{i}}\omega_{q,\lambda}^2}{2}\hat{\zeta}_{q,\lambda}\hat{\zeta}_{-q,-\lambda} + \frac{1}{2M_{\text{i}}}\hat{\pi}_{q,\lambda}\hat{\pi}_{-q,-\lambda}\right],\end{aligned} \tag{S.28}$$

and its expectation value satisfies $\langle \hat{\pi}_{\pm Q,\pm}\rangle = 0$. The phonon-related part of the mean-field Hamiltonian is given by

$$\begin{aligned}\hat{H}_{\mathrm{MF}}^{(\mathrm{ph})} &= \frac{M_{\mathrm{i}}\omega_{Q,+}^2}{2}\hat{\zeta}_{Q,+}^{\dagger}\hat{\zeta}_{Q,+} + \frac{2iQg_{\mathrm{T}}}{\sqrt{N_{\mathrm{i}}}}\langle \hat{S}_{-Q}^{(+)}\rangle \hat{\zeta}_{Q,+} + \mathrm{h.c.} \\ &= \frac{M_{\mathrm{i}}\omega_{Q,+}^2}{2}\left| \hat{\zeta}_{Q,+}^{\dagger} + \frac{2iQg_{\mathrm{T}}}{\sqrt{N_{\mathrm{i}}}M_{\mathrm{i}}\omega_{Q,+}^2}\langle \hat{S}_{-Q}^{(+)}\rangle\right|^2 - \frac{Q^2g_{\mathrm{T}}^2}{N_{\mathrm{i}}M_{\mathrm{i}}\omega_{Q,+}^2}|\langle \hat{S}_{-Q}^{(+)}\rangle|^2. \end{aligned} \tag{S.29}$$

Therefore, in the thermodynamically stable state, minimizing this energy yields the following condition.

$$\langle \hat{\zeta}_{Q,+}^{\dagger}\rangle + \frac{2iQg_{\mathrm{T}}}{\sqrt{N_{\mathrm{i}}}M_{\mathrm{i}}\omega_{Q,+}^2}\langle \hat{S}_{-Q}^{(+)}\rangle = 0. \tag{S.30}$$

Substituting the expression for $\langle \hat{S}_{-Q}^{(+)}\rangle$ and using the definition of the order parameter,

$$\Delta^* = -\frac{2iQg_{\mathrm{T}}}{\sqrt{N_{\mathrm{i}}}}\langle \hat{\zeta}_{Q,+}^{\dagger}\rangle, \tag{S.31}$$

we eventually obtain the self-consistent equation for the order parameter:

$$\begin{aligned}\Delta^* &= -\frac{4g_{\mathrm{T}}^2Q^2}{N_{\mathrm{i}}M_{\mathrm{i}}\omega_{Q,+}^2}\langle \hat{S}_{-Q}^{(+)}\rangle \\ &= \frac{4g_{\mathrm{T}}^2Q^2}{N_{\mathrm{i}}M_{\mathrm{i}}\omega_{Q,+}^2}\Delta^*\sum_k \frac{1}{2E_k}\left(1-2f(E_k)\right). \end{aligned} \tag{S.32}$$

This can be simplified as

$$1 = \frac{4g_{\mathrm{T}}^2Q^2}{M_{\mathrm{i}}\omega_{Q,+}^2}\cdot\frac{1}{N_{\mathrm{i}}}\sum_k \frac{1}{2E_k}\left(1-2f(E_k)\right). \tag{S.33}$$

The summation over the crystal momenta can be rewritten as

$$\begin{aligned}\frac{1}{N_{\mathrm{i}}}\sum_k \frac{1}{2E_k}\left(1-2f(E_k)\right) &= \frac{\Omega}{2\pi}\int dk\,\frac{1}{2E_k}\tanh\left(\frac{E_k}{2k_BT}\right) \\ &= \frac{\Omega}{4\pi\hbar v_F}\int_{-\epsilon_F}^{\epsilon_F} d\xi\,\frac{1}{\sqrt{\xi^2+|\Delta|^2}}\tanh\left(\frac{\sqrt{\xi^2+|\Delta|^2}}{2k_BT}\right), \end{aligned} \tag{S.34}$$

where $\Omega$ is the volume of the unit cell, and especially at zero temperature $T = 0$, we have

$$\begin{aligned}\frac{1}{N_{\mathrm{i}}}\sum_k \frac{1}{2E_k}\left(1-2f(E_k)\right) =& \frac{\Omega}{4\pi\hbar v_F}\int_{-\epsilon_F}^{\epsilon_F} d\xi\frac{1}{\sqrt{\xi^2+|\Delta|^2}} \\ =& \frac{\Omega}{2\pi\hbar v_F}\sinh^{-1}\left(\frac{\epsilon_F}{|\Delta|}\right). \end{aligned} \tag{S.35}$$

Thus, the above gap equation (S.33) can be rewritten as

$$\sinh^{-1}\left(\frac{\epsilon_F}{|\Delta|}\right) = \frac{\pi M_{\mathrm{i}}(\hbar\omega_{Q,+})^2}{8g_{\mathrm{T}}^2m_ek_F\Omega}. \tag{S.36}$$

Here, we define a dimensionless electron-phonon coupling constant by

$$\Lambda = \frac{8g_{\mathrm{T}}^2m_ek_F\Omega}{\pi M_{\mathrm{i}}(\hbar\omega_{Q,+})^2}. \tag{S.37}$$

Solving Eq. (S.36) allows us to express the Peierls gap at $T = 0$ as

$$\begin{aligned}|\Delta|_{T=0} =& \frac{\epsilon_F}{\sinh(1/\Lambda)} \\ \simeq& 2\epsilon_F\exp(-1/\Lambda), \end{aligned} \tag{S.38}$$

where the last approximation corresponds to the weak coupling limit. Meanwhile, the transition temperature obtained from the Green's function method is

$$T^{(\mathrm{TA})} = \frac{2e^{\gamma}}{\pi}\epsilon_F \exp(-1/\Lambda), \tag{S.39}$$

so that, similarly to BCS theory and conventional Peierls transitions, the universal ratio

$$\frac{\Delta_{T=0}}{T^{(\mathrm{TA})}} \sim 1.76. \tag{S.40}$$

also holds in our model. Note that, although we here considered the case at zero temperature $T = 0$, the same results can be derived by evaluating the free energy.

**5. Resultant orders in CISSPT.**

The spin density order per unit length (using $\hbar/2$ as the unit) can be expressed using the inverse Fourier transform as

$$\langle \hat{\boldsymbol{S}}(z)\rangle = \frac{1}{N_{\mathrm{i}}}\left\langle \sum_q \hat{\boldsymbol{S}}_q e^{iqz}\right\rangle, \tag{S.41}$$

from which we obtain

$$\langle \hat{S}_x(z)\rangle = \frac{1}{2N_{\mathrm{i}}}\left[\left\langle \hat{S}^{(+)}_{-Q}\right\rangle e^{-iQz} + \text{c.c.}\right] \tag{S.42}$$

$$= -\frac{|\Delta|}{2\pi\hbar v_F\Lambda}\cos(Qz+\phi), \tag{S.43}$$

and

$$\langle \hat{S}_y(z)\rangle = \frac{1}{2N_{\mathrm{i}}}\left[-i\left\langle \hat{S}^{(+)}_{-Q}\right\rangle e^{-iQz} + \text{c.c.}\right] \tag{S.44}$$

$$= \frac{|\Delta|}{2\pi\hbar v_F\Lambda}\sin(Qz+\phi). \tag{S.45}$$

Here, we used $\langle \hat{S}^{(+)}_{-Q}\rangle = \langle \hat{S}^{(-)}_{Q}\rangle^* = -\frac{N_{\mathrm{i}}}{2\pi\hbar v_F\Lambda}|\Delta|e^{-i\phi}$. Thus, the helical spin density wave in real space is given by

$$\delta\boldsymbol{S}(z) = \frac{|\Delta|}{2\pi\hbar v_F\Lambda}\begin{bmatrix}\cos(Qz+\phi)\\ -\sin(Qz+\phi)\\ 0\end{bmatrix}, \tag{S.46}$$

where the minus sign can be absorbed into the phase $\phi$ (i.e., $\phi \to \phi+\pi$), and can henceforth be regarded as a redefinition of $\phi$. For the other enantiomorph, the spin texture becomes

$$\delta\boldsymbol{S}(z) = \frac{|\Delta|}{2\pi\hbar v_F\Lambda}\begin{bmatrix}\cos(Qz+\phi)\\ \sin(Qz+\phi)\\ 0\end{bmatrix}. \tag{S.47}$$

At the same time, the condensation of soft phonon modes $(Q,+)$ and $(-Q,-)$ leads to a structural phase transition of the crystal. The resultant lattice distortion at each spatial point is given by

$$\begin{aligned}\delta\mathbf{u}(z) &= \frac{1}{\sqrt{N_{\mathrm{i}}}}\boldsymbol{\epsilon}_{Q,+}\langle\hat{\zeta}_{Q,+}\rangle e^{iQz} + \text{c.c.}\\ &= \frac{|\Delta|}{\sqrt{2}Qg_{\mathrm{T}}}\begin{bmatrix}\cos(Qz+\phi+\pi/2)\\ -\sin(Qz+\phi+\pi/2)\\ 0\end{bmatrix}.\end{aligned} \tag{S.48}$$

By aligning the definition of $\phi$ with that used in the helical SDW, the lattice displacement becomes

$$\delta\mathbf{u}(z) = \frac{|\Delta|}{\sqrt{2}Qg_{\mathrm{T}}}\begin{bmatrix}\cos(Qz+\phi-\pi/2)\\ -\sin(Qz+\phi-\pi/2)\\ 0\end{bmatrix}. \tag{S.49}$$

For the other enantiomorph, the lattice distortion becomes

$$\delta\mathbf{u}(z) = \frac{|\Delta|}{\sqrt{2Q g_{\mathrm{T}}}} \begin{bmatrix} \cos(Qz+\phi-\pi/2) \\ \sin(Qz+\phi-\pi/2) \\ 0 \end{bmatrix}. \tag{S.50}$$

**6. Commensurability effect in CISSPT.**

We have so far considered the physical properties realized by CISSPT with an incommensurate wave vector $Q$. In conventional CDWs and SDWs, it is well established that commensurability—when $Q$ forms a rational fraction of the lattice periodicity—qualitatively modifies the nature of the ordered state [29, 32–38]. For example, once the electronic ordering becomes commensurate, Umklapp processes lock the phase to the lattice, opening a gap in the phason spectrum and strongly altering collective motion. For CISSPT considered here, the role of commensurability is even more drastic. The nesting vector $(Q,+)$ couples the electronic states of $\hat{c}_{k,\downarrow}$ and $\hat{c}_{k+Q,\uparrow}$, while the nesting vector $(-Q,-)$ also couples the electronic states of $\hat{c}_{k-Q,\downarrow}$ and $\hat{c}_{k,\uparrow}$. In the incommensurate case, only $(k_F,\uparrow)$ and $(-k_F,\downarrow)$ states can be connected near the Fermi level, and these two couplings are equivalent. However, in the commensurate case, the states at $k$ and $k+NQ$ ($N$ integer) coincide, so that $\hat{c}_{k,\downarrow}$ and $\hat{c}_{k,\uparrow}$ can each couple to distinct electronic states. As a result, unlike in CDW or SDW systems, in the CISSPT the spin-selective gap-opening mechanism itself is prohibited in the commensurate case described below.

As before in this section, the case with soft modes $(Q,+)$ and $(-Q,-)$ is considered. In commensurate density waves, the wave vector $Q$ is a rational fraction of the lattice reciprocal vector $G=2\pi/c$, i.e., $Q/G=m/n$ with integers $m$ and $n$, which defines a superlattice with period $nc$. As a result, electronic states $k, k+Q, \ldots, k+(n-1)Q$ form a closed block that mixes all members, opening energy gaps not only at the Fermi level but also at multiple points across the BZ. This is in contrast to incommensurate waves, where no finite folding occurs, so only states near the Fermi surface experience significant gaps. Therefore, in a commensurate case we have to extend the minimal Hamiltonian fully including these states:

$$\hat{H}^{\mathrm{MF}}_{\mathrm{el}} = \sum_k \hat{\boldsymbol{C}}^\dagger_k \boldsymbol{H}^{(2n)}_k \hat{\boldsymbol{C}}_k, \tag{S.51}$$

$$\hat{\boldsymbol{C}}^\dagger_k = \begin{bmatrix} \hat{c}^\dagger_{k,\uparrow} & \hat{c}^\dagger_{k,\downarrow} & \hat{c}^\dagger_{k+Q,\uparrow} & \hat{c}^\dagger_{k+Q,\downarrow} \cdots & \hat{c}^\dagger_{k+(n-1)Q,\uparrow} & \hat{c}^\dagger_{k+(n-1)Q,\downarrow} \end{bmatrix}, \tag{S.52}$$

$$\boldsymbol{H}^{(2n)}_k = \begin{bmatrix} \boldsymbol{\xi}_k & \boldsymbol{\Delta} & & \cdots & \boldsymbol{\Delta}^\dagger \\ \boldsymbol{\Delta}^\dagger & \boldsymbol{\xi}_{k+Q} & \boldsymbol{\Delta} & \cdots & \\ & \boldsymbol{\Delta}^\dagger & \boldsymbol{\xi}_{k+2Q} & \cdots & \\ \vdots & & & \ddots & \boldsymbol{\Delta} \\ \boldsymbol{\Delta} & & & \boldsymbol{\Delta}^\dagger & \boldsymbol{\xi}_{k+(n-1)Q} \end{bmatrix}, \tag{S.53}$$

where $\boldsymbol{\xi}_k$ is the electronic Hamiltonian including spin degrees of freedom and, in CISSPT, the electronic states $(k,\downarrow)$ and $(k+Q,\uparrow)$ are coupled:

$$\boldsymbol{\Delta} = \begin{bmatrix} 0 & 0 \\ \Delta & 0 \end{bmatrix}. \tag{S.54}$$

The elements of this matrix can be explicitly written as

$$\boldsymbol{H}^{(2n)}_k = \begin{bmatrix} \xi_{k,\uparrow} & & & & & & \cdots & & \Delta^* \\ & \xi_{k,\downarrow} & \Delta & & & & \cdots & & \\ & \Delta^* & \xi_{k+Q,\uparrow} & & & & \cdots & & \\ & & & \xi_{k+Q,\downarrow} & \Delta & & \cdots & & \\ & & & \Delta^* & \xi_{k+2Q,\uparrow} & & \cdots & & \\ & & & & & \xi_{k+2Q,\downarrow} & \cdots & & \\ \vdots & \vdots & \vdots & \vdots & \vdots & \vdots & \ddots & \vdots & \vdots \\ & & & & & & \cdots & \xi_{k+(n-1)Q,\uparrow} & \\ \Delta & & & & & & \cdots & & \xi_{k+(n-1)Q,\downarrow} \end{bmatrix}. \tag{S.55}$$

Therefore, although the coupling in each sector is spin-selective, both the spin-up and spin-down electronic bands exhibit Peierls gaps, resulting in apparent electronic bands that are qualitatively the same as the conventional CDWs and SDWs.

For examples, we show the cases of half-filling and one-third filling in Supplementary Figs. S6 and S7. The mean field

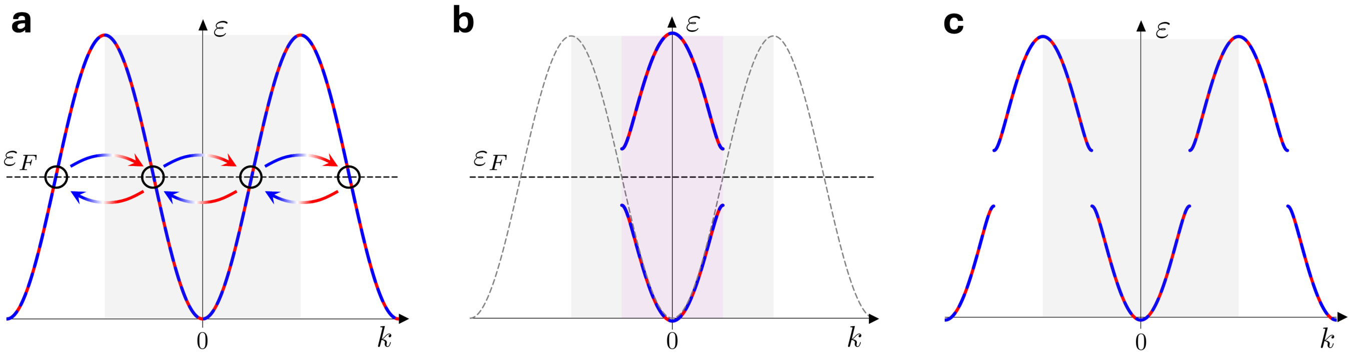


Supplementary Figure S6. **Schematic illustrations of electronic bands for the half-filling case**. **a**, The cosine-type and spin-degenerate electronic bands above the transition temperature. The grey shaded area represents the first BZ originating from the translational symmetry of the parent phase. The red-blue and blue-red gradient arrows couple the same electronic states shown by black circles, and connect both up and down spin sectors. **b**, The electronic bands below the transition temperature. The purple shaded area represents the reduced BZ folded by commensurate ordering vector $Q$. The grey dot line is the original electronic band. **c**, The unfolded electronic bands and Peierls gaps in the extended zone scheme.

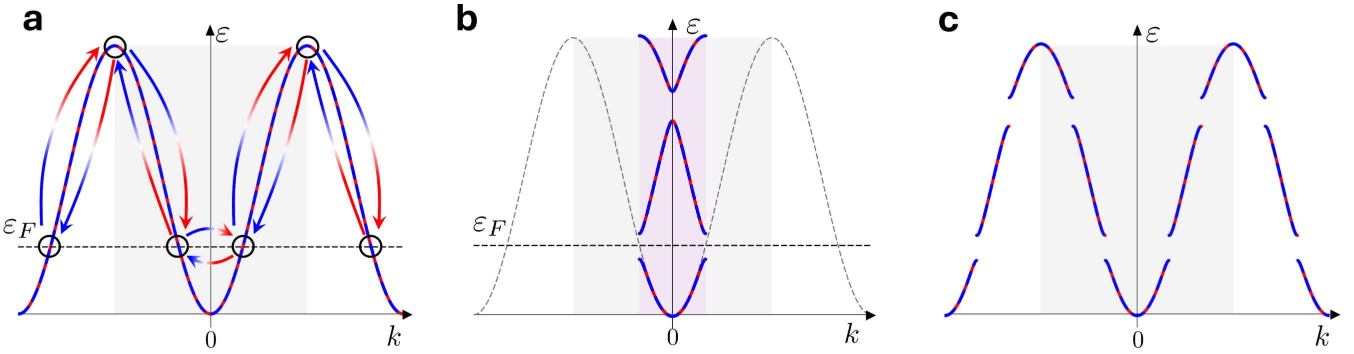


Supplementary Figure S7. **Schematic illustrations of electronic bands for the one-third filling case**. **a**, The electronic bands above the transition temperature. The electronic states $k-Q$, $k$, $k+Q$ are coupled. **b**, The electronic bands below the transition temperature. **c**, The unfolded electronic bands and Peierls gaps in the extended zone scheme.

Hamiltonian becomes

$$\boldsymbol{H}_k^{(4)} = \begin{bmatrix} \xi_{k,\downarrow} & \Delta & 0 & 0 \\ \Delta^* & \xi_{k+Q,\uparrow} & 0 & 0 \\ 0 & 0 & \xi_{k+Q,\downarrow} & \Delta \\ 0 & 0 & \Delta^* & \xi_{k,\uparrow} \end{bmatrix}, \tag{S.56}$$

for the half-filling case $Q/G = 1/2$, where we changed the basis so that the matrix becomes block-diagonalized. Moreover, since finite expectation values $\langle \hat{S}_{-Q}^{(+)} \rangle$ and $\langle \hat{S}_{-Q}^{(-)} \rangle$ coexist, the electronic order becomes the conventional collinear SDW:

$$\begin{aligned} \delta \boldsymbol{S}(z) &= \frac{|\Delta|}{2\pi\hbar v_F \Lambda} \begin{bmatrix} \cos(Qz+\phi) \\ -\sin(Qz+\phi) \\ 0 \end{bmatrix} + \frac{|\Delta|}{2\pi\hbar v_F \Lambda} \begin{bmatrix} \cos(Qz+\phi) \\ \sin(Qz+\phi) \\ 0 \end{bmatrix} \\ &= \frac{|\Delta|}{\pi\hbar v_F \Lambda} \cos(Qz+\phi) \boldsymbol{e}_x \\ &= \frac{|\Delta|}{\pi\hbar v_F \Lambda} \cos(\frac{\pi z}{c}+\phi) \boldsymbol{e}_x. \end{aligned} \tag{S.57}$$

In the half-filling case, the period of the density wave is precisely twice that of the lattice, and in other words, it results in antiferromagnetic ordering. The commensurability 2 is a particularly special case when we consider CISSPT. Since $2Q = G$, the softening of chiral phonons occurs at the BZ boundary where the phonon PAM is degenerate [22, 23]. Therefore, both $\hat{\zeta}_{Q,+}$

and $\hat{\zeta}_{Q,-}$ are frozen and, as a consequence, CISSPT no longer occurs. This fact is consistent with the results thus far. Note that, however, the absence of CISSPT due to commensurability is not confined to the half-filling case.

We also provide the Hamiltonian for commensurability 3 as an example:

$$\boldsymbol{H}_k^{(6)} = \begin{bmatrix} \xi_{k,\downarrow} & \Delta & 0 & 0 & 0 & 0 \\ \Delta^* & \xi_{k+Q,\uparrow} & 0 & 0 & 0 & 0 \\ 0 & 0 & \xi_{k+Q,\downarrow} & \Delta & 0 & 0 \\ 0 & 0 & \Delta^* & \xi_{k+2Q,\uparrow} & 0 & 0 \\ 0 & 0 & 0 & 0 & \xi_{k+2Q,\downarrow} & \Delta \\ 0 & 0 & 0 & 0 & \Delta^* & \xi_{k,\uparrow} \end{bmatrix}, \tag{S.58}$$

for the one-third filling case $Q/G = 1/3$.

From a graphical perspective, this characteristic can be understood more intuitively. Taking the case of half-filling as an example, the electronic state $(-k_F, \downarrow)$ is coupled to the state $(k_F, \uparrow)$ shown by the blue-red gradient arrow in Supplementary Fig. S6a. At the same time, the electronic state $(k_F, \downarrow)$ is coupled to the state $(3k_F, \uparrow)$, i.e., $(-k_F, \uparrow)$ in the first BZ. Therefore, the nesting vectors $(Q, +)$ and $(Q, -)$ coexist in the electronic states on the Fermi surface, and the up and down spin sectors couple identically. This holds at any gap position, and consequently, Peierls gaps open in both spin-up and down electronic bands.

## Supplementary Note 3. Derivation of collective excitations.

In this Supplementary note, we show the detailed calculations for the collective excitations in chirality-induced spin-selective Peierls states.

### 1. Calculations of phason and amplitudon frequencies

In conventional CDWs and SDWs, the primary collective excitations are phase fluctuations (phason) and amplitude fluctuations (amplitudon) of the density wave. Among them, the phason mode is of particular importance, as it underlies the sliding motion [29, 32, 33, 35, 39–41]. In CDWs, owing to the couplings with phonons, the effective masses of these modes are generally larger than the bare electron mass. This implies that the lattice follows the motion of the CDW. In contrast, the phason and amplitudon modes in SDWs are typically not coupled to phonons, and their effective masses in standard models remain comparable to the bare electron mass.

The Lee-Rice-Anderson model [41] can be applied for the calculation of the collective mode in CISSPT. Below the transition temperature, due to the presence of the nesting vector $Q$, phonons with wave vectors $Q+q$ and $-Q+q$ become hybridized. Therefore, in the Lee-Rice-Anderson model, the calculation within the RPA approximation is performed incorporating the density wave order. In the limit $\Delta \to 0$, this calculation coincides with the previous RPA calculation used to obtain the soft phonon mode. Since the notation can be somewhat confusing, we will continue to consider the soft modes $(Q,+)$ and $(-Q,-)$. In this case, the relevant contributions to the calculation come from the phonons with $(Q+q, \lambda=+1)$ and $(-Q+q, \lambda=-1)$, and the electronic states $(k+Q/2, s=+1/2)$ and $(k-Q/2, s=-1/2)$. Moreover, the sign of wave vector regions and spin (phonon angular momentum) are defined in the same manner as follows:

$$\hat{b}_{q+\alpha Q,\alpha}(\tau), \quad \hat{c}_{k+\alpha Q/2,\alpha/2}(\tau) \quad (\alpha=\pm). \tag{S.59}$$

By employing a formulation similar to the anomalous Green function, the electron Green function is redefined as

$$\mathscr{G}_{\alpha\beta}(k,\tau) = -\langle T(\hat{c}_{k+\alpha Q/2,\alpha/2}(\tau)\hat{c}^{\dagger}_{k+\beta Q/2,\beta/2})\rangle \quad (\alpha,\beta=\pm). \tag{S.60}$$

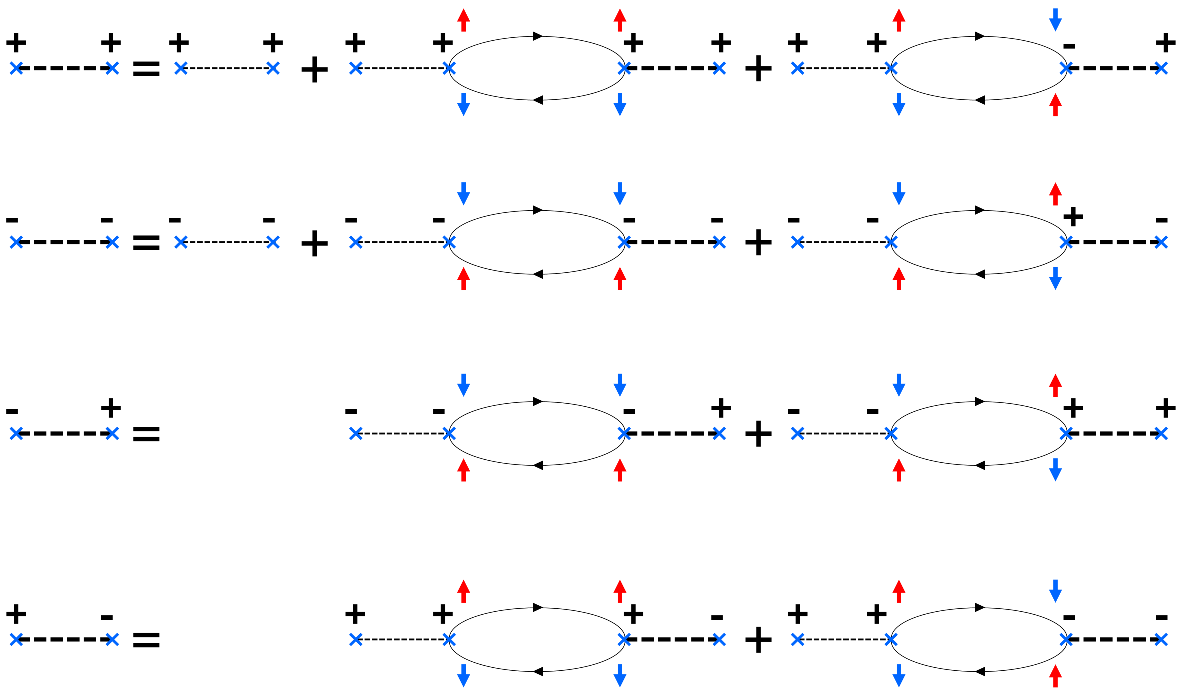

Supplementary Figure S8. **Feynman diagram for the Lee-Rice-Anderson model in CISSPT.** The blue crosses represent the vertex part for $\hat{H}^{(\mathrm{T})}_{\mathrm{ep}}$. The red and blue arrows indicate spin up and down, respectively. The $+$ and $-$ denote the sign of the coupled phonon wave vector Q, that is, $\alpha$.

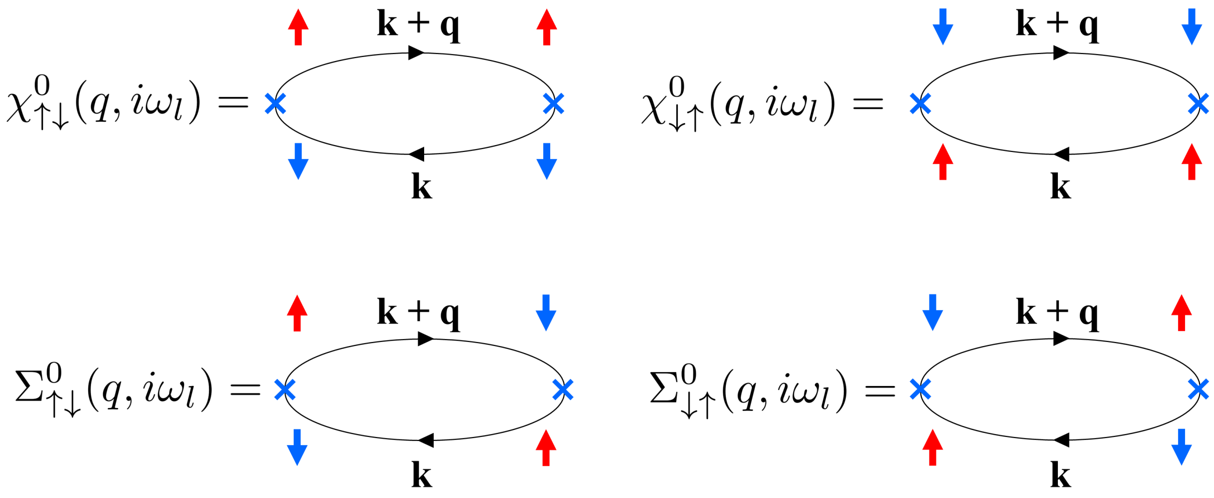


Supplementary Figure S9. **Feynman diagram defining phonon self-energy**.

Defining, as in the Nambu representation for superconductors,

$$\Psi_k = \begin{bmatrix} \hat{c}_{k+Q/2,\uparrow} \\ \hat{c}_{k-Q/2,\downarrow} \end{bmatrix}, \quad \Psi_k^\dagger = \begin{bmatrix} \hat{c}^\dagger_{k+Q/2,\uparrow} & \hat{c}^\dagger_{k-Q/2,\downarrow} \end{bmatrix}, \tag{S.61}$$

the Green function is expressed in matrix form as

$$\boldsymbol{\mathcal{G}}(k,\tau) = \begin{bmatrix} -\langle T(\hat{c}_{k+Q/2,\uparrow}(\tau)\hat{c}^\dagger_{k+Q/2,\uparrow})\rangle & -\langle T(\hat{c}_{k+Q/2,\uparrow}(\tau)\hat{c}^\dagger_{k-Q/2,\downarrow})\rangle \\ -\langle T(\hat{c}_{k-Q/2,\downarrow}(\tau)\hat{c}^\dagger_{k+Q/2,\uparrow})\rangle & -\langle T(\hat{c}_{k-Q/2,\downarrow}(\tau)\hat{c}^\dagger_{k-Q/2,\downarrow})\rangle \end{bmatrix}. \tag{S.62}$$

The inverse matrix is computed as follows:

$$\boldsymbol{\mathcal{G}}^{-1}(k,i\epsilon_n) = i\epsilon_n \boldsymbol{I} - \boldsymbol{H}_k = \begin{bmatrix} i\epsilon_n - \xi_{k+Q/2,\uparrow} & -\Delta \\ -\Delta^* & i\epsilon_n - \xi_{k-Q/2,\downarrow} \end{bmatrix}, \tag{S.63}$$

thus, we obtain

$$\boldsymbol{\mathcal{G}}(k,i\epsilon_n) = (\det \boldsymbol{\mathcal{G}})^{-1} \begin{bmatrix} i\epsilon_n - \xi_{k-Q/2,\downarrow} & \Delta \\ \Delta^* & i\epsilon_n - \xi_{k+Q/2,\uparrow} \end{bmatrix}. \tag{S.64}$$

$$\det \boldsymbol{\mathcal{G}} \simeq (i\epsilon_n)^2 - E_k^2. \tag{S.65}$$

Similarly, the phonon Green function is redefined as

$$\boldsymbol{\mathcal{D}}_{\alpha\beta}(q,\tau) = -\langle T(\hat{b}_{\alpha Q+q,\alpha}(\tau) + \hat{b}^\dagger_{-\alpha Q-q,-\alpha}(\tau))(\hat{b}_{-\beta Q-q,-\beta} + \hat{b}^\dagger_{\beta Q+q,\beta})\rangle. \tag{S.66}$$

From the above notation, the Dyson equations under the RPA shown in Supplementary Fig. S8 are as follows.

$$\begin{aligned}
\boldsymbol{\mathcal{D}}_{++}(q,i\omega_l) =& \boldsymbol{\mathcal{D}}^{(0)}_{++}(q,i\omega_l) + \boldsymbol{\mathcal{D}}^{(0)}_{++}(q,i\omega_l)\chi^{(0)}_{\uparrow\downarrow}(q,i\omega_l)\boldsymbol{\mathcal{D}}_{++}(q,i\omega_l) + \boldsymbol{\mathcal{D}}^{(0)}_{++}(q,i\omega_l)\Sigma^{(0)}_{\uparrow\downarrow}(q,i\omega_l)\boldsymbol{\mathcal{D}}_{+-}(q,i\omega_l),\\
\boldsymbol{\mathcal{D}}_{--}(q,i\omega_l) =& \boldsymbol{\mathcal{D}}^{(0)}_{--}(q,i\omega_l) + \boldsymbol{\mathcal{D}}^{(0)}_{--}(q,i\omega_l)\chi^{(0)}_{\downarrow\uparrow}(q,i\omega_l)\boldsymbol{\mathcal{D}}_{--}(q,i\omega_l) + \boldsymbol{\mathcal{D}}^{(0)}_{--}(q,i\omega_l)\Sigma^{(0)}_{\downarrow\uparrow}(q,i\omega_l)\boldsymbol{\mathcal{D}}_{-+}(q,i\omega_l),\\
\boldsymbol{\mathcal{D}}_{+-}(q,i\omega_l) =& \boldsymbol{\mathcal{D}}^{(0)}_{--}(q,i\omega_l)\chi^{(0)}_{\downarrow\uparrow}(q,i\omega_l)\boldsymbol{\mathcal{D}}_{+-}(q,i\omega_l) + \boldsymbol{\mathcal{D}}^{(0)}_{--}(q,i\omega_l)\Sigma^{(0)}_{\downarrow\uparrow}(q,i\omega_l)\boldsymbol{\mathcal{D}}_{++}(q,i\omega_l),\\
\boldsymbol{\mathcal{D}}_{-+}(q,i\omega_l) =& \boldsymbol{\mathcal{D}}^{(0)}_{++}(q,i\omega_l)\chi^{(0)}_{\uparrow\downarrow}(q,i\omega_l)\boldsymbol{\mathcal{D}}_{-+}(q,i\omega_l) + \boldsymbol{\mathcal{D}}^{(0)}_{++}(q,i\omega_l)\Sigma^{(0)}_{\uparrow\downarrow}(q,i\omega_l)\boldsymbol{\mathcal{D}}_{--}(q,i\omega_l),
\end{aligned}$$

where we redefined each bubble term as

$$\begin{aligned}
\chi^{(0)}_{\uparrow\downarrow}(q,i\omega_l) =& \frac{k_BT}{N}\sum_{k,i\epsilon_n}|g^{(\mathrm{T})}_{\uparrow\downarrow}(Q,+)|^2\boldsymbol{\mathcal{G}}^{(0)}_{++}(k+q,i\epsilon_n+i\omega_l)\boldsymbol{\mathcal{G}}^{(0)}_{--}(k,i\epsilon_n),\\
\chi^{(0)}_{\downarrow\uparrow}(q,i\omega_l) =& \frac{k_BT}{N}\sum_{k,i\epsilon_n}|g^{(\mathrm{T})}_{\downarrow\uparrow}(Q,-)|^2\boldsymbol{\mathcal{G}}^{(0)}_{--}(k+q,i\epsilon_n+i\omega_l)\boldsymbol{\mathcal{G}}^{(0)}_{++}(k,i\epsilon_n),\\
\Sigma^{(0)}_{\uparrow\downarrow}(q,i\omega_l) =& \frac{k_BT}{N}\sum_{k,i\epsilon_n}|g^{(\mathrm{T})}_{\uparrow\downarrow}(Q,+)|^2\boldsymbol{\mathcal{G}}^{(0)}_{-+}(k+q,i\epsilon_n+i\omega_l)\boldsymbol{\mathcal{G}}^{(0)}_{-+}(k,i\epsilon_n),\\
\Sigma^{(0)}_{\downarrow\uparrow}(q,i\omega_l) =& \frac{k_BT}{N}\sum_{k,i\epsilon_n}|g^{(\mathrm{T})}_{\downarrow\uparrow}(Q,-)|^2\boldsymbol{\mathcal{G}}^{(0)}_{+-}(k+q,i\epsilon_n+i\omega_l)\boldsymbol{\mathcal{G}}^{(0)}_{+-}(k,i\epsilon_n).
\end{aligned}$$

These bubble parts of electron-hole parings are shown in Supplementary Fig. S9. In the region where the wave vectors $k$ and $q$ are small, the following relations

$$\begin{aligned}
\xi_{k+Q/2\uparrow} = \xi_{-k-Q/2\downarrow} = -\xi_{-k+Q/2\uparrow} = -\xi_{k-Q/2\downarrow},\\
\boldsymbol{\mathcal{G}}^{(0)}_{++}(k,i\epsilon_n) = \boldsymbol{\mathcal{G}}^{(0)}_{--}(-k,i\epsilon_n) = -\boldsymbol{\mathcal{G}}^{(0)}_{--}(k,-i\epsilon_n),
\end{aligned}$$

approximately hold. Therefore, the following symmetries exist between the electronic bubble terms;

$$\begin{aligned}
\chi^{(0)}_{\uparrow\downarrow}(q,i\omega_l) =& \chi^{(0)}_{\downarrow\uparrow}(q,i\omega_l),\\
\Sigma^{(0)}_{\uparrow\downarrow}(q,i\omega_l) =& \Sigma^{(0)}_{\downarrow\uparrow}(q,i\omega_l),
\end{aligned}$$

which also lead to the following relation for the phonon Green function from the Dyson equations.

$$\begin{aligned}
\boldsymbol{\mathcal{D}}_{++}(q,i\omega_l) =& \boldsymbol{\mathcal{D}}_{--}(q,i\omega_l),\\
\boldsymbol{\mathcal{D}}_{+-}(q,i\omega_l) =& \boldsymbol{\mathcal{D}}_{-+}(q,i\omega_l).
\end{aligned}$$

Consequently, only the Dyson equations for $\boldsymbol{\mathcal{D}}_{++}(q,i\omega_l)$ and $\boldsymbol{\mathcal{D}}_{+-}(q,i\omega_l)$ need to be solved. Note that in the limit of $\Delta\to 0$, $\boldsymbol{\mathcal{D}}_{++}(q,i\omega_l)$ agrees with the diagram for soft phonons, while $\boldsymbol{\mathcal{D}}_{+-}(q,i\omega_l)$ represents the effect of the folded BZ associated with the Peierls transition. By solving the Dyson equations, we finally obtain

$$\begin{aligned}
\boldsymbol{\mathcal{D}}_{++}(q,i\omega_l)+\boldsymbol{\mathcal{D}}_{+-}(q,i\omega_l) =& \frac{1}{\mathcal{D}^{(0)}(Q,i\omega_l)^{-1}-\chi^{(0)}(q,i\omega_l)-\Sigma^{(0)}(q,i\omega_l)},\\
\boldsymbol{\mathcal{D}}_{++}(q,i\omega_l)-\boldsymbol{\mathcal{D}}_{+-}(q,i\omega_l) =& \frac{1}{\mathcal{D}^{(0)}(Q,i\omega_l)^{-1}-\chi^{(0)}(q,i\omega_l)+\Sigma^{(0)}(q,i\omega_l)},
\end{aligned}$$

where we approximated $\omega_{q\pm Q}\simeq\omega_{\pm Q}$, i.e., defined $\mathcal{D}^{(0)}(Q,i\omega_l)\equiv\mathscr{D}^{(0)}_{\mathrm{T}}(Q,+,i\omega_l)$.

The frequencies of phason and amplitudon are determined in the same manner as in the Lee-Rice-Anderson model, described by the pole of

$$A_\pm(q,\omega) = \frac{1}{2}(\boldsymbol{\mathcal{D}}_{++}(q,\omega)\pm\boldsymbol{\mathcal{D}}_{+-}(q,\omega)).$$

The $\boldsymbol{\mathcal{D}}_{++}+\boldsymbol{\mathcal{D}}_{+-}$ mode corresponds to the amplitude fluctuation, while the $\boldsymbol{\mathcal{D}}_{++}-\boldsymbol{\mathcal{D}}_{+-}$ mode corresponds to the phase fluctuation [41]. This fact can be understood simply in terms of small oscillations of the phonon field around the mean field $\hat{\zeta}_0$. The fluctuation of the phonon field is decomposed as $\hat{\zeta}_{\pm Q}\simeq(\hat{\zeta}_0+\delta\hat{\zeta})e^{\pm i\delta\phi}$ with the amplitude fluctuation $\delta\hat{\zeta}$ and the phase fluctuation $\delta\phi$. Then, to the lowest order of fluctuations, $\hat{\zeta}_Q+\hat{\zeta}_{-Q}=2(\hat{\zeta}_0+\delta\hat{\zeta})$ and $\hat{\zeta}_Q-\hat{\zeta}_{-Q}=2i\delta\phi$ are satisfied. Each quantity describes the fluctuation, and therefore $\boldsymbol{\mathcal{D}}_{++}\pm\boldsymbol{\mathcal{D}}_{+-}$ correspond to the amplitude and phase fluctuation modes, which are illustrated in Figs. S10a and b.

The explicit calculation shows the following dispersions of the amplitude and phase modes,

$$\Omega^2_+(q) = \Lambda\omega^2_{Q,+}+\frac{1}{3}\frac{m_e}{m^*_e}v^2_Fq^2,$$

$$\Omega^2_-(q) = \frac{m_e}{m^*_e}v^2_Fq^2, \tag{S.67}$$

$$m^*_e \equiv m_e\left(1+\frac{4|\Delta|^2}{\Lambda(\hbar\omega_{Q,+})^2}\right), \tag{S.68}$$

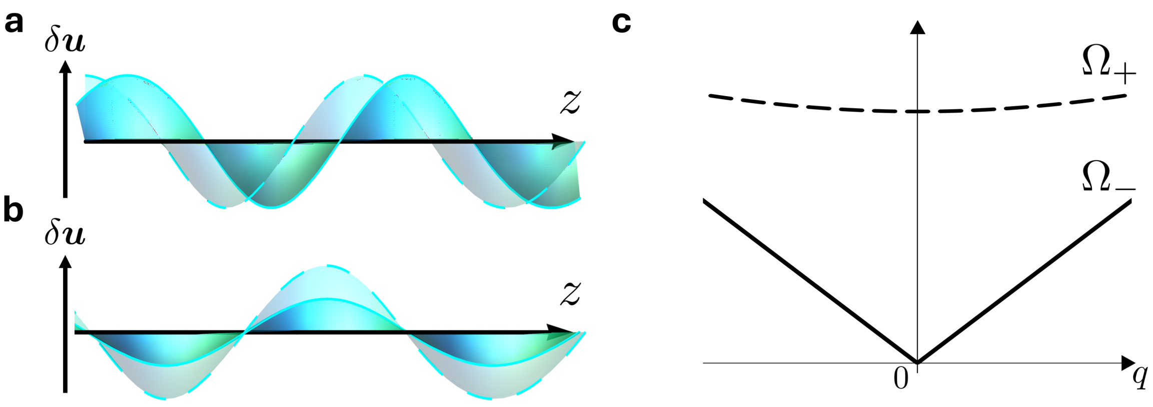


Supplementary Figure S10. **Collective modes in incommensurate CISSPT**. **a**, Schematic image of the phase mode (phason). **b**, Schematic image of the amplitude mode (amplitudon). **c**, The energy dispersions of the phason $\Omega_-$ and the amplitudon $\Omega_+$.

which are shown in Fig. S10c. Here, $m_e^*$ is the effective mass reflecting the nature of CISSPT, where chiral phonons couple with electrons, and the response time becomes slower than that of bare electrons. The amplitudon mode $\Omega_+(q)$ is a gapful optical mode. Meanwhile, the phason mode $\Omega_-(q) \sim q$ is the Goldstone mode and contributes to the sliding motion of the density wave.

## Supplementary Note 4. On transverse Peierls transitions and chiral charge density waves.

In the main text and Supplementary Notes 1-3, we have discussed CISSPT, taking the EPC Hamiltonian,

$$\hat{H}_{\rm ep}^{(\rm T)} = \frac{1}{\sqrt{N}} \sum_{k,q,s,s'} \sum_{\lambda=\pm} iqg_T \hat{c}^{\dagger}_{k+q,s} \hat{c}_{k,s'} \hat{\zeta}_{q,\,\lambda} \delta_{s,\,s'+l^{\rm ph}_{z,\lambda}}, \tag{S.69}$$

as our starting point (see Methods). However, tracing back to its origins, this expression is the minimal Hamiltonian derived from Eq. (S.9). Therefore, another minimal model can be considered, such as the following process that preserves electron spin:

$$\hat{H}_{\rm ep}^{(\rm T)} = \frac{1}{\sqrt{N}} \sum_{k,q,m_{\rm orb},m'_{\rm orb}} \sum_{\lambda=\pm} iqg_T \hat{c}^{\dagger}_{k+q,m_{\rm orb}} \hat{c}_{k,m'_{\rm orb}} \hat{\zeta}_{q,\,\lambda} \delta_{m_{\rm orb},m'_{\rm orb}+l^{\rm ph}_{z,\lambda}}. \tag{S.70}$$

We remind $\delta_{m_{\rm orb},m'_{\rm orb}+l^{\rm ph}_{z,\lambda}}$ in this article means $m_{\rm orb} = m'_{\rm orb} + l^{\rm ph}_{z,\lambda} \mod n$. In this case, instead of the spin-flip process, coupling arises between the real-space component of the electron PAM $m_{\rm orb}$ and the phonon PAM. Similarly to the CISSPT, this type of EPC also induces softening dependent on phonon chirality. However, it results in transverse Peierls transitions and chiral charge density waves. In this Supplementary Note 4, we briefly discuss the transverse Peierls transition. We also show the emergence of a novel class of chiral charge density waves. Hereafter, the spin index is omitted for simplicity.

### 1. Transverse Peierls transitions in chiral crystals.

We first mention that the EPC of Eq. (S.70) is equivalent to that derived from the tight-binding model in Ref. [2], both satisfying the conservation law of total PAM. Unlike the transverse Peierls transition discussed in Ref. [15], the phonon dispersions here remain intrinsically non-degenerate because we focus on the Peierls transition in chiral crystals.

We here consider the system with three-fold screw symmetry, that is, electronic PAM $m_{\rm orb} \in \{0, \pm 1\}$ and phonon PAM $l^{\rm ph}_{z,\lambda} \in \{0, \pm 1\}$. In the Peierls transition, the time-reversal pair $(k_F, m_{\rm orb})$, $(-k_F, -m_{\rm orb})$ is coupled by the phonon scattering. In accordance with the conservation law of total PAM, the following equation holds in the $\hat{S}_3$ system.

$$m_{\rm orb} \equiv -m_{\rm orb} + l^{\rm ph}_{z,\lambda} \mod 3, \tag{S.71}$$

which reduces to the compact form;

$$2\, m_{\rm orb} \equiv l^{\rm ph}_{z,\lambda} \mod 3. \tag{S.72}$$

Therefore, the Kohn anomaly of chiral phonon with $l^{\rm ph}_{z,\lambda} = 1$ corresponds to the Peierls instability between the $(k_F, -1)$ and $(-k_F, 1)$ electronic states. In the same manner, the chiral phonon with $l^{\rm ph}_{z,\lambda} = -1$ corresponds to the Peierls instability between the $(k_F, 1)$ and $(-k_F, -1)$ states. This is analogous to the spin-flip process discussed in Supplementary Note 2 and the main text, and we only have to extend it to the multiband formulation.

Following the same procedure as in Supplementary Note 2, the phonon self-energy contributed by electron particle–hole excitations reads

$$\Pi^{(\rm T)}(q, +, i\omega_m) = \frac{2\hbar q^2 g_{\rm T}^2}{M_{\rm i}\omega_{q,+}} \chi^{(0)}_{-1,\,1}(q, i\omega_m), \tag{S.73}$$

$$\Pi^{(\rm T)}(q, -, i\omega_m) = \frac{2\hbar q^2 g_{\rm T}^2}{M_{\rm i}\omega_{q,-}} \chi^{(0)}_{1,\,-1}(q, i\omega_m), \tag{S.74}$$

with the bare electron self-energy

$$\chi^{(0)}_{m_{\rm orb},-m_{\rm orb}}(q, i\omega_m) = \frac{k_B T}{N_{\rm i}} \sum_{k,i\epsilon_n} \mathscr{G}^{(0)}_{m_{\rm orb}}(k, i\epsilon_n)\, \mathscr{G}^{(0)}_{-m_{\rm orb}}(k-q, i\epsilon_n - i\omega_m), \tag{S.75}$$

where $\mathscr{G}^{(0)}_{\rm orb}(k, i\epsilon_n) = (i\epsilon_n - \xi_{k,m_{\rm orb}})^{-1}$ is the Green function for the electron with band index $m_{\rm orb}$. The phonon's self-energy in Eqs. (S.73) and (S.74) still depends on the chiral phonon frequency $\omega_{q,\lambda}$. Therefore, if phonon softening occurs in the transverse modes, the transition temperature differs for each handedness of the chiral phonon. This is the mechanism of chirality-dependent Kohn anomaly discussed in Supplementary Note 2, here realized in the electronic PAM channel.

When the phonon modes $(Q, \lambda)$ and $(-Q, -\lambda)$ are frozen, the order parameter is defined by the same form as in the main text, $\Delta = 2iQg_T\langle\hat{\zeta}_{Q,+}\rangle/\sqrt{N_{\rm i}}$. The electronic order parameter that acquires a finite expectation value is the inter-band density operator,

$$\hat{\rho}_Q^{(m_{\rm orb},-m_{\rm orb})} \equiv \sum_k \hat{c}^{\dagger}_{k+Q,m_{\rm orb}}\, \hat{c}_{k,-m_{\rm orb}}. \tag{S.76}$$

We hereafter assume that the soft phonon modes are $(Q, \lambda)$ and $(-Q, -\lambda)$ with the incommensurate wave vector $Q$ and introduce $2\,\ell \equiv l^{\rm ph}_{z,\lambda} \mod 3$, i.e., $(\lambda,\, \ell) = (1, -1)$ or $(-1, 1)$. The relevant electronic bands near the Fermi level $(k_F, \ell)$ and $(-k_F, -\ell)$ construct a $2 \times 2$ minimal Hamiltonian. Defining the spinor

$$\hat{\boldsymbol{C}}_k^\dagger = \left[\hat{c}^\dagger_{k,\,\ell} \ \ \hat{c}^\dagger_{k-Q,\,-\ell}\right], \tag{S.77}$$

the mean-field Hamiltonian becomes

$$\hat{H}^{\rm MF}_{\rm el} = \sum_{k>0} \hat{\boldsymbol{C}}_k^\dagger \begin{bmatrix} \xi_{k,\,\ell} & \Delta \\ \Delta^* & \xi_{k-Q,\,-\ell} \end{bmatrix} \hat{\boldsymbol{C}}_k. \tag{S.78}$$

Accordingly, the eigenenergy is given by

$$E_\pm(k) = \frac{\xi_{k,\,\ell} + \xi_{k-Q,\,-\ell}}{2} \pm \sqrt{\left(\frac{\xi_{k,\,\ell} - \xi_{k-Q,\,-\ell}}{2}\right)^2 + |\Delta|^2}. \tag{S.79}$$

We now obtain the real-space charge modulation by projecting the expectation value onto the real-space density operator. In complete analogy with Supplementary Note 2, the electronic density operator and $\Delta$ are connected by the following linear relation.

$$\left\langle \hat{\rho}_Q^{(\ell,-\ell)} \right\rangle = \frac{N_i}{2\pi\hbar v_F \Lambda}\,\Delta^*, \tag{S.80}$$

where $\Lambda$ is the dimensionless electron-phonon coupling constant. On the other hand, when explicitly incorporating the Bloch function and band index (here, the degrees of freedom of the electronic PAM), the electronic density is given as follows.

$$\begin{aligned} \hat{\rho}(\mathbf{r}) =& \Psi^\dagger(\boldsymbol{r})\Psi(\boldsymbol{r}) \\ =& \sum_{m_{\rm orb}, m'_{\rm orb}} \sum_{k,k'} \hat{c}^\dagger_{k,m_{\rm orb}} \hat{c}_{k',m'_{\rm orb}}\, u^*_{k,m_{\rm orb}}(z) u_{k',m'_{\rm orb}}(z)\, e^{i(k'-k)z} e^{i(m'_{\rm orb}-m_{\rm orb})\Phi}. \end{aligned} \tag{S.81}$$

By retaining the non-zero dominant finite-$Q$ component generated by the $(\ell, -\ell)$ off-diagonal expectation value, we have

$$\begin{aligned} \langle \hat{\rho}(\mathbf{r}) \rangle =& \sum_k \left\langle \hat{\rho}_Q^{(\ell,-\ell)} \right\rangle F_\ell\, e^{-iQz} e^{-i\cdot 2\ell\Phi} + \text{c.c.}, \\ &\propto |\Delta| \cos(Qz - 2\ell\Phi + \phi). \end{aligned} \tag{S.82}$$

We defined the form factor

$$F_\ell \equiv \frac{1}{V_{\rm cell}} \int dz\, u^*_{k+Q,\ell}(z)\, u_{k,-\ell}(z), \tag{S.83}$$

and assumed that the $k$-dependence of $F_\ell$ is negligible for brevity. To avoid confusion, we note that $\phi$ denotes the initial phase of the density wave, while $\Phi = \tan^{-1}(y/x)$ denotes the azimuthal angle within the $xy$ plane. Alongside, the lattice displacement follows from the phonon condensate and results in the chiral standing wave:

$$\delta\mathbf{u}(z) = \frac{|\Delta|}{\sqrt{2}\,Q g_T} \begin{bmatrix} \sin(Qz+\phi) \\ -\lambda\cos(Qz+\phi) \\ 0 \end{bmatrix}, \tag{S.84}$$

which is the same form as calculated in Supplementary Note 2.

This result indicates that the system experiences a chiral charge density wave associated with the transverse Peierls transition. The charge density given by Eq. (S.82) shows that the charge density wave is not a simple one-dimensional modulation $\cos(Qz)$, but rather a helical pattern with an additional winding structure $e^{\pm i2\ell\Phi}$ in the azimuthal coordinate. A close analogy is optical vortex beams [42, 43], where the factor $e^{i2\ell\Phi}$ endows photons with orbital angular momentum $2\ell\hbar$. Another analog are cholesteric liquid crystals [44, 45]. The charge density wave therefore becomes spiral order with the periodicity $2\pi/Q$ wrapped around the $z$-axis, with which the chiral lattice distortion possessing the same period emerges.

At the same time, the charge density wave preserves the $2\ell$-fold rotational symmetry, $\hat{C}_{2\ell}$, which originates from the inherent electronic PAM. Therefore, as shown in Supplementary Fig. S11, the charge alignment exhibits electric multipole order within each $xy$ plane and rotates along the $z$-axis direction. In addition, we remark that this class of chiral CDW is entirely different

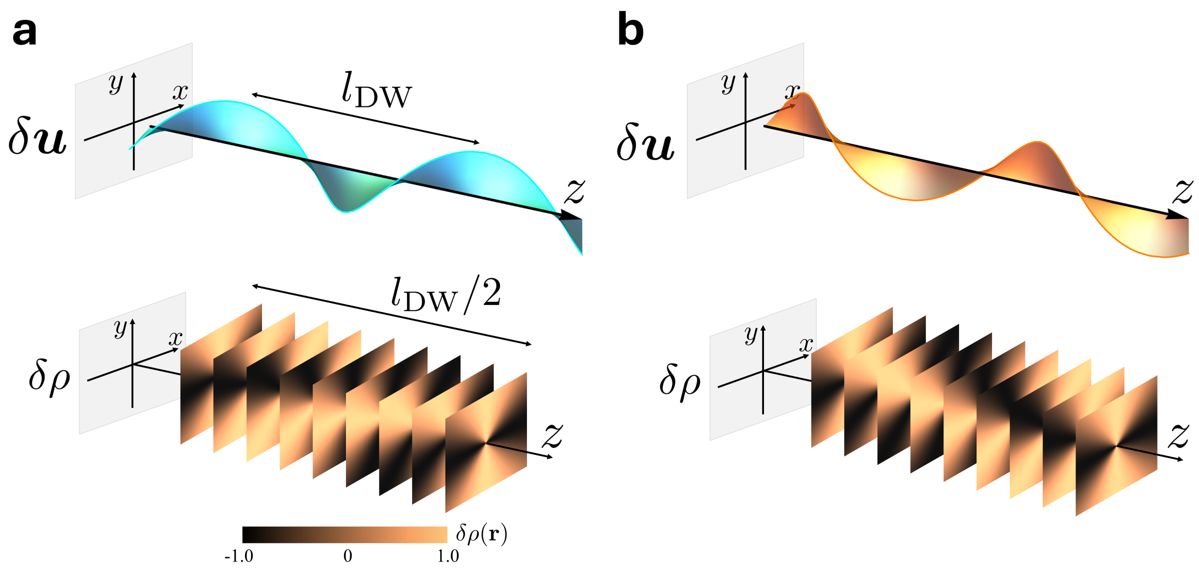


Supplementary Figure S11. **Winding charge density waves and entailed lattice distortions**. **a**, The chiral lattice distortion (top) and winding charge density wave (bottom), associated with transverse Peierls transition in the LH crystal. The color bar represents the modulation of charge density $\delta\rho(\mathbf{r})$, and we see that electric quadrupolar modulation rotates counter-clockwise along the $z$-axis. For clarity, we show only half a period of the winding CDW. **b**, The same figure as **a**, but in the RH crystal. The charge density wave rotates clockwise along the $z$-axis.

from chiral CDWs observed recently in van der Waals materials [46–55]: the former comes from a single wave vector and becomes twisted itself, while the latter originates from multiple wave number vectors, each of which is arranged by rotating relative to one another. In order to distinguish between these orders, we here refer to the CDW discussed above as a winding CDW.

In the $\hat{S}_3$ symmetric systems, determined by the handedness of the reference crystal, the pair of $(\lambda, \ell)$ takes the values of $(1, -1)$ or $(-1, 1)$. By substituting these values into Eqs. (S.82) and (S.84), the concrete azimuth-dependence of the ordered states becomes

$$\langle\hat{\rho}(\mathbf{r})\rangle \propto |\Delta| \cos(Qz + 2\Phi + \phi) \equiv \delta\rho_R(\mathbf{r}), \tag{S.85}$$

$$\delta\mathbf{u}(z) \propto |\Delta| \begin{bmatrix} \sin(Qz+\phi) \\ -\cos(Qz+\phi) \\ 0 \end{bmatrix}, \tag{S.86}$$

for the right-handed crystals based on the notation in the main text and

$$\langle\hat{\rho}(\mathbf{r})\rangle \propto |\Delta| \cos(Qz - 2\Phi + \phi) \equiv \delta\rho_L(\mathbf{r}), \tag{S.87}$$

$$\delta\mathbf{u}(z) \propto |\Delta| \begin{bmatrix} \sin(Qz+\phi) \\ \cos(Qz+\phi) \\ 0 \end{bmatrix}, \tag{S.88}$$

for the left-handed crystals. In particular, the crystals with $\hat{S}_3$ symmetry host the $\hat{C}_2$-preserving (i.e., electric quadrupolar) winding CDW. Furthermore, the chirality, that is, the direction of the spiral in the winding CDW $\langle\hat{\rho}(\mathbf{r})\rangle$ and the lattice distortion $\delta\mathbf{u}(z)$ is inverted among the opposite enantiomorphs because the signs of $\lambda$ and $\ell\,(= m_{\rm orb})$ reverse between the right-handed and left-handed crystals.

We again emphasize the winding CDW,

$$\delta\rho_R(\mathbf{r}) = |\Delta| \cos(Qz + 2\Phi), \tag{S.89}$$

is chiral. Its chiral nature is revealed by checking how $\delta\rho(\mathbf{r})$ transforms under spatial symmetries. The transformation properties under inversion, mirror, and rotation operations are summarized below:

- **Inversion** ($\mathbf{r} \to -\mathbf{r}$): $\cos(Qz + 2\Phi) \to \cos(Qz - 2\Phi) \quad (\because\ \Phi \to \Phi + \pi, z \to -z)$
- **Mirror in yz-plane** ($x \to -x$): $\cos(Qz + 2\Phi) \to \cos(Qz - 2\Phi) \quad (\because\ \Phi \to \pi - \Phi, z \to z)$

- **Mirror in xz-plane** ($y \to -y$): $\cos(Qz + 2\Phi) \to \cos(Qz - 2\Phi) \quad (\because \Phi \to -\Phi, z \to z)$
- **Diagonal mirror x = y** ($x \leftrightarrow y$): $\cos(Qz + 2\Phi) \to \cos(Qz - 2\Phi) \quad (\because \Phi \to \pi/2 - \Phi, z \to z)$
- **Diagonal mirror x = -y** ($x \leftrightarrow -y$): $\cos(Qz - 2\Phi) \to \cos(Qz - 2\Phi) \quad (\because \Phi \to -\pi/2 - \Phi, z \to z)$
- **180° rotation about z** ($C_{2,z}$): $\cos(Qz + 2\Phi) \to \cos(Qz + 2\Phi) \quad (\because \Phi \to \Phi + \pi, z \to z)$
- **180° rotation about x** ($C_{2,x}$): $\cos(Qz + 2\Phi) \to \cos(Qz + 2\Phi) \quad (\because \Phi \to -\Phi, z \to -z)$
- **180° rotation about y** ($C_{2,y}$): $\cos(Qz + 2\Phi) \to \cos(Qz + 2\Phi) \quad (\because \Phi \to \pi - \Phi, z \to -z)$

Here, we set the initial phase as $\phi = 0$. These rules show that all mirror and inversion symmetries are broken, while $\hat{C}_2$ rotation around the $z$-axis is preserved. Consequently, the azimuthal dependence encodes a well-defined handedness, confirming that the charge modulation $\delta\rho(\mathbf{r})$ is intrinsically chiral, which in turn indicates that the winding CDW is characterized by a proper pseudo-scalar. For example, by the analogy of the vortex beam, $\ell$ in Eq. (S.82) corresponds to the topological charge of the vortex beam. Therefore, chiral characteristics of the winding CDW, i.e., $G_0$ interpretation, can be expressed by a product of the wave vector $Q$ and the winding number of phase $\ell$ (see Methods).

**2. Collective excitations and angular momentum transport**

The above formulation can be straightforwardly extended to the discussion of the collective excitations associated with the ordered phase. Importantly, since the lattice displacement field $\delta u$ takes exactly the same form as in the CISSPT of the main text, the dynamical properties of the collective modes directly entail the circular motion of ions. Consequently, the sliding motion of the chiral density wave leads to a mechanical angular momentum flow, which is consistent with Ref. [15].

Moreover, the winding CDW carries a winding number $2\ell$, indicating that the density modulation itself belongs to a finite angular momentum channel. As a result, the sliding motion of the winding CDW also transports not only linear momentum (as in conventional CDWs) but also a well-defined flux of orbital angular momentum [42, 43]. This orbital angular momentum character provides a direct bridge between electronic ordering phenomena and the broader context of vortex physics in wave systems.

**3. Coexistence of CISSPT and chiral charge density wave order**

We comment on the possible coexistence of CISSPT and chiral CDWs. At the most fundamental level, the selection rule imposed by the conservation law of the total PAM is

$$l_{\text{PAM,el}} = l'_{\text{PAM,el}} + l^{s}_{\text{PAM,ph}} \mod n, \tag{S.90}$$

which we assumed to be decoupled as

$$m_{\text{orb}} + s = m'_{\text{orb}} + s' + l^{\text{ph}}_{z,\lambda} \mod n. \tag{S.91}$$

Depending on how the chiral phonon mediates transitions between electronic states, either the electronic spin sector (discussed in the main text) or the orbital sector (discussed in Supplementary Note 4) of PAM - or most significantly both simultaneously - can contribute to the Peierls instability.

This observation implies that a winding CDW and a helical SDW are not mutually exclusive but may emerge cooperatively within the same microscopic framework. Such coexistence enriches the variety of possible ordered states and highlights the central role of chiral phonons in unifying spin, orbital, and lattice degrees of freedom.

**4. Extension to transverse Peierls transitions in achiral crystals.**

Throughout this article, we have focused on chiral crystals, where the screw symmetry endows the electrons and phonons with well-defined pseudo angular momentum. This symmetry guarantees strict selection rules, and the resulting coupling between electronic bands and chiral phonons naturally drives transverse Peierls transitions such as the CISSPT and a winding CDW. This concept is not limited to chiral crystals. If anything, our results can naturally be extended to a more general form with $n$-fold rotational symmetry $\hat{C}_n$. In this case, the role of pseudo angular momentum is naturally replaced by the orbital angular momentum or, more strictly, by the discrete angular momentum associated with the underlying rotational symmetry $\hat{C}_n$ [13, 24, 56, 57]. This replacement immediately generalizes the framework of Ref. [15], where the selection rule of the phonon angular momentum and electron spins was invoked, to the rigorous conservation including electronic orbital angular momentum.

The crucial difference between chiral and achiral crystals is that, in the latter, phonons carrying opposite angular momenta are generically degenerate. As pointed out by Ref. [15], if this degeneracy is lifted either intrinsically or extrinsically, the system undergoes a transverse Peierls transition accompanied by chiral CDWs. In this achiral case, the azimuthal dependence of the winding CDW that was governed by electronic PAM in chiral systems [$\ell$ in Eq. (S.82)] is instead determined by the orbital (or

discrete) angular momentum of the electronic bands. Therefore, extending our model can naturally reveal $C_2$- and $C_4$-symmetric chiral CDWs [58], linking the symmetry of the density wave order to the underlying electronic angular momentum.

---

* asano.shun.57x@st.kyoto-u.ac.jp
† yanase@scphys.kyoto-u.ac.jp

[1] X. Wang, Y. Xian, and Y. Yan, Chiral electrons and spin selectivity at chiral-achiral interfaces (2024), arXiv:2306.01664 [cond-mat.mtrl-sci].

[2] T. Tateishi, A. Kato, and J.-i. Kishine, Electron–chiral phonon coupling, crystal angular momentum, and phonon chirality, Journal of the Physical Society of Japan **94**, 053601 (2025).

[3] I. Božovic, Possible band-structure shapes of quasi-one-dimensional solids, Phys. Rev. B **29**, 6586 (1984).

[4] W. Izumida, K. Sato, and R. Saito, Spin–orbit interaction in single wall carbon nanotubes: Symmetry adapted tight-binding calculation and effective model analysis, Journal of the Physical Society of Japan **78**, 074707 (2009).

[5] D. Gosálbez-Martínez, A. Crepaldi, and O. V. Yazyev, Diversity of radial spin textures in chiral materials, Phys. Rev. B **108**, L201114 (2023).

[6] M. Sakano, M. Hirayama, T. Takahashi, S. Akebi, M. Nakayama, K. Kuroda, K. Taguchi, T. Yoshikawa, K. Miyamoto, T. Okuda, K. Ono, H. Kumigashira, T. Ideue, Y. Iwasa, N. Mitsuishi, K. Ishizaka, S. Shin, T. Miyake, S. Murakami, T. Sasagawa, and T. Kondo, Radial spin texture in elemental tellurium with chiral crystal structure, Phys. Rev. Lett. **124**, 136404 (2020).

[7] J. A. Krieger, S. Stolz, I. Robredo, K. Manna, E. C. McFarlane, M. Date, B. Pal, J. Yang, E. B. Guedes, J. H. Dil, C. M. Polley, M. Leandersson, C. Shekhar, H. Borrmann, Q. Yang, M. Lin, V. N. Strocov, M. Caputo, M. D. Watson, T. K. Kim, C. Cacho, F. Mazzola, J. Fujii, I. Vobornik, S. S. P. Parkin, B. Bradlyn, C. Felser, M. G. Vergniory, and N. B. M. Schröter, Weyl spin-momentum locking in a chiral topological semimetal, Nature Communications **15**, 3720 (2024).

[8] G. Chang, B. J. Wieder, F. Schindler, D. S. Sanchez, I. Belopolski, S.-M. Huang, B. Singh, D. Wu, T.-R. Chang, T. Neupert, S.-Y. Xu, H. Lin, and M. Z. Hasan, Topological quantum properties of chiral crystals, Nature Materials **17**, 978 (2018).

[9] K. Ishito, H. Mao, Y. Kousaka, Y. Togawa, S. Iwasaki, T. Zhang, S. Murakami, J.-i. Kishine, and T. Satoh, Truly chiral phonons in $\alpha$-hgs, Nature Physics **19**, 35 (2023).

[10] T. Zhang and S. Murakami, Chiral phonons and pseudoangular momentum in nonsymmorphic systems, Phys. Rev. Res. **4**, L012024 (2022).

[11] Y. Yang, Z. Xiao, Y. Mao, Z. Li, Z. Wang, T. Deng, Y. Tang, Z.-D. Song, Y. Li, H. Yuan, M. Shi, and Y. Xu, Catalogue of chiral phonon materials (2025), arXiv:2506.13721 [cond-mat.mtrl-sci].

[12] S. Zhang, Z. Huang, M. Du, T. Ying, L. Du, and T. Zhang, Comprehensive study of phonon chirality under symmetry constraints (2025), arXiv:2503.22794 [cond-mat.mtrl-sci].

[13] H. Zhu, J. Yi, M.-Y. Li, J. Xiao, L. Zhang, C.-W. Yang, R. A. Kaindl, L.-J. Li, Y. Wang, and X. Zhang, Observation of chiral phonons, Science **359**, 579 (2018).

[14] X. Chen, X. Lu, S. Dubey, Q. Yao, S. Liu, X. Wang, Q. Xiong, L. Zhang, and A. Srivastava, Entanglement of single-photons and chiral phonons in atomically thin wse2, Nature Physics **15**, 221 (2019).

[15] K. Luo and X. Dai, Transverse peierls transition, Phys. Rev. X **13**, 011027 (2023).

[16] G. L. Bir and G. E. Pikus, Symmetry and strain-induced effects in semiconductors (Wiley, 1974).

[17] J. Fransson, Chiral phonon induced spin polarization, Phys. Rev. Res. **5**, L022039 (2023).

[18] J. Fransson, Vibrational origin of exchange splitting and "chiral-induced spin selectivity, Phys. Rev. B **102**, 235416 (2020).

[19] D. S. L. Abergel and V. I. Fal'ko, Spin-orbit-assisted electron-phonon interaction and the magnetophonon resonance in semiconductor quantum wells, Phys. Rev. B **77**, 035317 (2008).

[20] A. Kumar, P. Chandra, and P. A. Volkov, Spin-phonon resonances in nearly polar metals with spin-orbit coupling, Phys. Rev. B **105**, 125142 (2022).

[21] A. Kumar, P. Chandra, and P. A. Volkov, Phonon-induced collective modes in spin-orbit coupled polar metals, Phys. Rev. B **108**, 075162 (2023).

[22] H. Tsunetsugu and H. Kusunose, Theory of energy dispersion of chiral phonons, Journal of the Physical Society of Japan **92**, 023601 (2023).

[23] A. Kato and J.-i. Kishine, Note on angular momentum of phonons in chiral crystals, Journal of the Physical Society of Japan **92**, 075002 (2023).

[24] T. Wang, H. Sun, X. Li, and L. Zhang, Chiral phonons: Prediction, verification, and application, Nano Letters **24**, 4311 (2024).

[25] H. Ueda, M. García-Fernández, S. Agrestini, C. P. Romao, J. van den Brink, N. A. Spaldin, K.-J. Zhou, and U. Staub, Chiral phonons in quartz probed by x-rays, Nature **618**, 946 (2023).

[26] H. Chen, W. Wu, J. Zhu, Z. Yang, W. Gong, W. Gao, S. A. Yang, and L. Zhang, Chiral phonon diode effect in chiral crystals, Nano Letters **22**, 1688 (2022).

[27] J. Kishine, A. S. Ovchinnikov, and A. A. Tereshchenko, Chirality-induced phonon dispersion in a noncentrosymmetric micropolar crystal, Phys. Rev. Lett. **125**, 245302 (2020).

[28] A. A. Abrikosov, I. Dzyaloshinskii, L. P. Gorkov, and R. A. Silverman, Methods of quantum field theory in statistical physics (Dover, New York, NY, 1975).

[29] G. Grüner, Density Waves In Solids, 1st ed. (CRC Press, 1994).

[30] A. Manchon, H. C. Koo, J. Nitta, S. M. Frolov, and R. A. Duine, New perspectives for rashba spin–orbit coupling, Nature Materials **14**,

871 (2015).
[31] V. Galitski and I. B. Spielman, Spin–orbit coupling in quantum gases, Nature **494**, 49 (2013).
[32] G. Grüner, The dynamics of charge-density waves, Rev. Mod. Phys. **60**, 1129 (1988).
[33] G. Grüner, The dynamics of spin-density waves, Rev. Mod. Phys. **66**, 1 (1994).
[34] P. M. and, Electronic crystals: an experimental overview, Advances in Physics **61**, 325 (2012).
[35] G. Grüner and A. Zettl, Charge density wave conduction: A novel collective transport phenomenon in solids, Physics Reports **119**, 117 (1985).
[36] A. J. Berlinsky, One-dimensional metals and charge density wave effects in these materials, Reports on Progress in Physics **42**, 1243 (1979).
[37] D. Radić, Charge density waves in solids—from first concepts to modern insights, Symmetry **17**, 10.3390/sym17071135 (2025).
[38] E. Fawcett, Spin-density-wave antiferromagnetism in chromium, Rev. Mod. Phys. **60**, 209 (1988).
[39] H. Seo, C. Hotta, and H. Fukuyama, Toward systematic understanding of diversity of electronic properties in low-dimensional molecular solids, Chemical Reviews **104**, 5005 (2004).
[40] H. Fukuyama and P. A. Lee, Dynamics of the charge-density wave. i. impurity pinning in a single chain, Phys. Rev. B **17**, 535 (1978).
[41] P. Lee, T. Rice, and P. Anderson, Conductivity from charge or spin density waves, Solid State Communications **14**, 703 (1974).
[42] K. Bliokh, I. Ivanov, G. Guzzinati, L. Clark, R. Van Boxem, A. Béché, R. Juchtmans, M. Alonso, P. Schattschneider, F. Nori, and J. Verbeeck, Theory and applications of free-electron vortex states, Physics Reports **690**, 1 (2017), theory and applications of free-electron vortex states.
[43] S. M. Lloyd, M. Babiker, G. Thirunavukkarasu, and J. Yuan, Electron vortices: Beams with orbital angular momentum, Rev. Mod. Phys. **89**, 035004 (2017).
[44] X. Zhang, Y. Xu, C. Valenzuela, X. Zhang, L. Wang, W. Feng, and Q. Li, Liquid crystal-templated chiral nanomaterials: from chiral plasmonics to circularly polarized luminescence, Light: Science & Applications **11**, 223 (2022).
[45] D. Andrienko, Introduction to liquid crystals, Journal of Molecular Liquids **267**, 520 (2018), special Issue Dedicated to the Memory of Professor Y. Reznikov.
[46] J. Ishioka, Y. H. Liu, K. Shimatake, T. Kurosawa, K. Ichimura, Y. Toda, M. Oda, and S. Tanda, Chiral charge-density waves, Phys. Rev. Lett. **105**, 176401 (2010).
[47] H. F. Yang, K. Y. He, J. Koo, S. W. Shen, S. H. Zhang, G. Liu, Y. Z. Liu, C. Chen, A. J. Liang, K. Huang, M. X. Wang, J. J. Gao, X. Luo, L. X. Yang, J. P. Liu, Y. P. Sun, S. C. Yan, B. H. Yan, Y. L. Chen, X. Xi, and Z. K. Liu, Visualization of chiral electronic structure and anomalous optical response in a material with chiral charge density waves, Phys. Rev. Lett. **129**, 156401 (2022).
[48] K. Kim, H.-W. J. Kim, S. Ha, H. Kim, J.-K. Kim, J. Kim, J. Kwon, J. Seol, S. Jung, C. Kim, D. Ishikawa, T. Manjo, H. Fukui, A. Q. R. Baron, A. Alatas, A. Said, M. Merz, M. Le Tacon, J. M. Bok, K.-S. Kim, and B. J. Kim, Origin of the chiral charge density wave in transition-metal dichalcogenide, Nature Physics **20**, 1919 (2024).
[49] J. van Wezel, Chirality and orbital order in charge density waves, Europhysics Letters **96**, 67011 (2011).
[50] W. Shi, B. J. Wieder, H. L. Meyerheim, Y. Sun, Y. Zhang, Y. Li, L. Shen, Y. Qi, L. Yang, J. Jena, P. Werner, K. Koepernik, S. Parkin, Y. Chen, C. Felser, B. A. Bernevig, and Z. Wang, A charge-density-wave topological semimetal, Nature Physics **17**, 381 (2021).
[51] Y. Zhao, Z. Nie, H. Hong, X. Qiu, S. Han, Y. Yu, M. Liu, X. Qiu, K. Liu, S. Meng, L. Tong, and J. Zhang, Spectroscopic visualization and phase manipulation of chiral charge density waves in 1t-tas2, Nature Communications **14**, 2223 (2023).
[52] S. Shao, W.-C. Chiu, M. S. Hossain, T. Hou, N. Wang, I. Belopolski, Y. Zhao, J. Ni, Q. Zhang, Y. Li, J. Liu, M. Yahyavi, Y. Jin, Q. Feng, P. Cui, C.-L. Zhang, Y. Yao, Z. Wang, J.-X. Yin, S.-Y. Xu, Q. Ma, W. bo Gao, A. Bansil, M. Z. Hasan, and G. Chang, A predictive first-principles framework of chiral charge density waves (2024), arXiv:2411.03664 [cond-mat.mtrl-sci].
[53] X. Luo, D. Obeysekera, C. Won, S. H. Sung, N. Schnitzer, R. Hovden, S.-W. Cheong, J. Yang, K. Sun, and L. Zhao, Ultrafast modulations and detection of a ferro-rotational charge density wave using time-resolved electric quadrupole second harmonic generation, Phys. Rev. Lett. **127**, 126401 (2021).
[54] B. Singh, G. McNamara, K.-M. Kim, S. Siddique, S. D. Funni, W. Zhang, X. Luo, P. Sakrikar, E. M. Kenney, R. Singha, S. Alekseev, S. A. A. Ghorashi, T. J. Hicken, C. Baines, H. Luetkens, Y. Wang, V. M. Plisson, M. Geiwitz, C. A. Occhialini, R. Comin, M. J. Graf, L. Zhao, J. Cano, R. M. Fernandes, J. J. Cha, L. M. Schoop, and K. S. Burch, Ferroaxial density wave from intertwined charge and orbital order in rare-earth tritellurides, Nature Physics **21**, 1578 (2025).
[55] D. Wulferding, J. Park, T. Tohyama, S. R. Park, and C. Kim, Magnetic field control over the axial character of higgs modes in charge-density wave compounds, Nature Communications **16**, 114 (2025).
[56] L. Zhang and Q. Niu, Angular momentum of phonons and the einstein–de haas effect, Phys. Rev. Lett. **112**, 085503 (2014).
[57] L. Zhang and Q. Niu, Chiral phonons at high-symmetry points in monolayer hexagonal lattices, Phys. Rev. Lett. **115**, 115502 (2015).
[58] F. Z. Yang, K. F. Luo, W. Zhang, X. Guo, W. R. Meier, H. Ni, H. X. Li, P. Mercado Lozano, G. Fabbris, A. H. Said, C. Nelson, T. T. Zhang, A. F. May, M. A. McGuire, R. Juneja, L. Lindsay, H. N. Lee, J.-M. Zuo, M. F. Chi, X. Dai, L. Zhao, and H. Miao, Incommensurate transverse peierls transition and signature of chiral charge density wave in eual4, Nature Communications **16**, 10401 (2025).
